# Supplementary material for: Long-Horizon AI Research for Grothendieck Constant: A Case Study in Human-AI Mathematical Collaboration
Source: arXiv:2608.11195 source file (2026-08-14)
Supplement: Supplementary file 3 [file certification_new_appendix_v2.tex]

% Insert this section after \appendix in paper/appendix.tex.
\section{Certification details}
\label{app:certification-details}

This appendix proves Proposition~\ref{prop:certified-numerical-input}.  The
first computation encloses the coefficient head through degree $251$.  The
second bounds the single boundary norm
$\|D^3H\|_{L^2(\mathbb T)}$ used in
Lemma~\ref{lem:third-order-tail}.

\subsection{The coefficient head}
\label{app:certification-coefficient-head}

Let $W,X$ be independent standard Gaussians and write
\[
  f(w,x)=\operatorname{sgn}\bigl(w+\vartheta\operatorname{He}_3(x)\bigr).
\]
For $a,b\ge0$, define
\[
  A_{a,b}
  :=\mathbb E\bigl[f(W,X)\operatorname{He}_a(W)
  \operatorname{He}_b(X)\bigr].
\]
As shown in Section~4, if
\[
  \rho(t)=\frac{t-s_3^2t^3+s_5^2t^5}{1+s_3^2+s_5^2},
\]
then
\begin{equation}
  H(t)=\frac{\pi}{2}\sum_{a,b\ge0}A_{a,b}^2\rho(t)^a(-t)^b,
  \label{eq:appendix-correlation-expansion}
\end{equation}
and hence
\begin{equation}
  b_m=\frac{\pi}{2}
  \sum_{\substack{a,b\ge0\\a+b\le m}}
  (-1)^bA_{a,b}^2[t^{m-b}]\rho(t)^a.
  \label{eq:appendix-coefficient-formula}
\end{equation}

The coefficients $A_{a,b}$ reduce to one-dimensional Gaussian integrals.  If
$Z$ is standard Gaussian and
\[
  q_a(u):=\mathbb E[\operatorname{sgn}(Z+u)\operatorname{He}_a(Z)],
\]
then
\[
  A_{a,b}
  =\mathbb E\bigl[\operatorname{He}_b(X)
  q_a(\vartheta\operatorname{He}_3(X))\bigr],
\]
where
\[
  q_0(u)=\operatorname{erf}\!\left(\frac{u}{\sqrt2}\right),
  \qquad
  q_a(u)=\frac{2\varphi(u)}{\sqrt a}
  \operatorname{He}_{a-1}(-u)
  \quad(a\ge1).
\]
Each integral is enclosed by outward-rounded adaptive quadrature on a finite
interval, together with a closed Gaussian-tail estimate.  Finite coefficient
extraction in \eqref{eq:appendix-coefficient-formula} then gives
\begin{equation}
  b_1\ge0.881573822049,
  \qquad
  \sum_{\substack{3\le m\le251\\m\ \mathrm{odd}}}|b_m|
  \le1.1328860\cdot10^{-5}.
  \label{eq:appendix-head-output}
\end{equation}

\subsection{A boundary representation of $D^3H$}
\label{app:certification-boundary-representation}

For real $|r|<1$, let
\[
  K_r(u,v)
  :=\frac{1}{2\pi\sqrt{1-r^2}}
  \exp\!\left(-\frac{u^2-2ruv+v^2}{2(1-r^2)}\right)
\]
be the centered bivariate Gaussian density with correlation $r$.  Let
$C_r(x,y)$ denote the conditional sign-correlation kernel
\[
  C_r(x,y)
  :=\frac{\pi}{2}\,
  \mathbb E\!\left[
  \operatorname{sgn}(W+\vartheta\operatorname{He}_3(x))
  \operatorname{sgn}(W'+\vartheta\operatorname{He}_3(y))
  \right],
\]
where $(W,W')$ is a standard Gaussian pair with correlation $r$.
The two derivative identities needed below follow directly from the Hermite
expansion of this kernel.

\begin{lemma}[Differentiating the threshold-correlation kernel]
\label{lem:appendix-kernel-differentiation}
For real $|r|<1$,
\begin{align}
  \partial_rC_r(x,y)
  &=2\pi K_r\bigl(\vartheta\operatorname{He}_3(x),
                   \vartheta\operatorname{He}_3(y)\bigr),
  \label{eq:appendix-kernel-r}\\
  \partial_x\partial_yC_r(x,y)
  &=2\pi\vartheta^2\operatorname{He}_3'(x)
  \operatorname{He}_3'(y)
  K_r\bigl(\vartheta\operatorname{He}_3(x),
           \vartheta\operatorname{He}_3(y)\bigr).
  \label{eq:appendix-kernel-xy}
\end{align}
\end{lemma}

\begin{proof}
Put
\[
  u=\vartheta\operatorname{He}_3(x),
  \qquad
  v=\vartheta\operatorname{He}_3(y).
\]
The Hermite covariance identity gives
\begin{equation}
  C_r(x,y)=\frac{\pi}{2}\sum_{a\ge0}r^a q_a(u)q_a(v),
  \label{eq:appendix-Cr-Hermite}
\end{equation}
where $q_a$ is the one-dimensional threshold coefficient defined above.  The
series and its $r$-derivative converge locally uniformly for $|r|<1$.  For
$a\ge1$,
\[
  q_a(u)=\frac{2\varphi(u)}{\sqrt a}\operatorname{He}_{a-1}(-u).
\]
Consequently,
\begin{align*}
  \partial_rC_r(x,y)
  &=\frac{\pi}{2}\sum_{a\ge1}a r^{a-1}q_a(u)q_a(v)\\
  &=2\pi\varphi(u)\varphi(v)
    \sum_{n\ge0}r^n\operatorname{He}_n(-u)
                         \operatorname{He}_n(-v).
\end{align*}
Mehler's identity identifies the last expression with $2\pi K_r(u,v)$,
proving \eqref{eq:appendix-kernel-r}.

Differentiating the defining integral for $q_a$ gives, for every $a\ge0$,
\[
  q_a'(u)=2\varphi(u)\operatorname{He}_a(-u).
\]
Differentiating \eqref{eq:appendix-Cr-Hermite} in $x$ and $y$ and applying
Mehler's identity once more yields
\begin{align*}
  \partial_x\partial_yC_r(x,y)
  &=\frac{\pi}{2}\vartheta^2\operatorname{He}_3'(x)
    \operatorname{He}_3'(y)
    \sum_{a\ge0}r^a q_a'(u)q_a'(v)\\
  &=2\pi\vartheta^2\operatorname{He}_3'(x)
    \operatorname{He}_3'(y)K_r(u,v),
\end{align*}
which proves \eqref{eq:appendix-kernel-xy}.
\end{proof}

Thus, after one derivative, the discontinuous sign functions are replaced by
explicit smooth Gaussian kernels.  The formulas above initially hold for
$|r|<1$; the explicit Gaussian expressions provide the analytic continuation
used on the complex curve $r=\rho(e^{i\theta})$ below.

If $\Psi$ has Hermite coefficients $\widehat\Psi_{i,j}$, define the diagonal
trace
\[
  T_\lambda[\Psi]
  :=\widehat\Psi_{0,0}+\sum_{n\ge1}\lambda^n\widehat\Psi_{n,n},
  \qquad |\lambda|\le1.
\]
For $|\lambda|<1$, this is the expectation of $\Psi(X,Y)$ when $(X,Y)$ is a
standard Gaussian pair with correlation $\lambda$.

\begin{lemma}[Differentiating the diagonal trace]
\label{lem:appendix-trace-differentiation}
If $\Psi(t)$ is a sufficiently regular family of kernels, then for $|t|<1$,
\begin{equation}
  D_tT_{-t}[\Psi(t)]
  =T_{-t}\!\left[D_t\Psi(t)-t\partial_x\partial_y\Psi(t)\right],
  \qquad D_t=t\partial_t.
  \label{eq:appendix-trace-differentiation}
\end{equation}
\end{lemma}

\begin{proof}
Write
\[
  \Psi(t;x,y)=\sum_{i,j\ge0}\widehat\Psi_{i,j}(t)
  \operatorname{He}_i(x)\operatorname{He}_j(y).
\]
Since $D_t(-t)^n=n(-t)^n$, termwise differentiation gives
\[
  D_tT_{-t}[\Psi(t)]
  =T_{-t}[D_t\Psi(t)]
   +\sum_{n\ge1}n(-t)^n\widehat\Psi_{n,n}(t).
\]
The identity
$\frac{d}{dx}\operatorname{He}_n(x)=\sqrt n\operatorname{He}_{n-1}(x)$
shows that
\[
  -tT_{-t}[\partial_x\partial_y\Psi(t)]
  =\sum_{n\ge1}n(-t)^n\widehat\Psi_{n,n}(t).
\]
Combining the last two displays proves
\eqref{eq:appendix-trace-differentiation}.
\end{proof}

The Cauchy--Schwarz inequality gives the boundary trace estimate
\begin{equation}
  |T_\lambda[\Psi]|
  \le
  \|\Psi\|_{L^2(\mu)}
  +\frac{\pi}{\sqrt6}
  \|\partial_x\partial_y\Psi\|_{L^2(\mu)},
  \label{eq:appendix-trace-bound}
\end{equation}
where $\mu$ is product standard Gaussian measure.

For $|t|<1$, one has
\[
  H(t)=T_{-t}[C_{\rho(t)}].
\]
Define
\[
  \Phi_0(t;x,y):=C_{\rho(t)}(x,y),
  \qquad
  \Phi_{k+1}:=D_t\Phi_k-t\partial_x\partial_y\Phi_k.
\]
Applying the differentiation identity three times gives
\begin{equation}
  D^3H(t)=T_{-t}[\Phi_3(t;\cdot,\cdot)].
  \label{eq:appendix-D3-trace}
\end{equation}
The interval bounds below provide a uniform integrable majorant, which
justifies taking radial limits in \eqref{eq:appendix-D3-trace} as
$|t|\uparrow1$.

\subsection{The nine smooth kernels}
\label{app:certification-nine-kernels}

Write $\rho_j=D_t^j\rho$.  For $p+a\ge1$, set
\[
  G_{p,a}(t;x,y)
  :=\left[
  \partial_r^p(\partial_x\partial_y)^aC_r(x,y)
  \right]_{r=\rho(t)}.
\]
Expanding the recursion before taking norms gives
\[
  \Phi_3(t;x,y)
  =\sum_{(p,a)\in\mathcal I}c_{p,a}(t)G_{p,a}(t;x,y),
\]
where
\[
  \mathcal I=
  \{(1,0),(2,0),(3,0),(0,1),(0,2),(0,3),
    (1,1),(2,1),(1,2)\},
\]
and
\begin{center}
\begin{tabular}{c c@{\qquad}c c}
\toprule
$(p,a)$ & $c_{p,a}(t)$ & $(p,a)$ & $c_{p,a}(t)$\\
\midrule
$(1,0)$ & $\rho_3$ & $(0,1)$ & $-t$\\
$(2,0)$ & $3\rho_1\rho_2$ & $(0,2)$ & $3t^2$\\
$(3,0)$ & $\rho_1^3$ & $(0,3)$ & $-t^3$\\
$(1,1)$ & $-3t(\rho_1+\rho_2)$ & $(2,1)$ & $-3t\rho_1^2$\\
$(1,2)$ & $3t^2\rho_1$ & & \\
\bottomrule
\end{tabular}
\end{center}

Define
\begin{align*}
  Q^{(0)}_{p,a}
  &:=\frac{1}{2\pi}\int_0^{2\pi}
  |c_{p,a}(e^{i\theta})|^2
  \|G_{p,a}(e^{i\theta})\|_2^2\,d\theta,\\
  Q^{(1)}_{p,a}
  &:=\frac{1}{2\pi}\int_0^{2\pi}
  |c_{p,a}(e^{i\theta})|^2
  \|\partial_x\partial_yG_{p,a}(e^{i\theta})\|_2^2\,d\theta.
\end{align*}
The trace estimate \eqref{eq:appendix-trace-bound} and Minkowski's inequality
give
\begin{equation}
  \|D^3H\|_{L^2(\mathbb T)}
  \le
  \sum_{(p,a)\in\mathcal I}\sqrt{Q^{(0)}_{p,a}}
  +\frac{\pi}{\sqrt6}
  \sum_{(p,a)\in\mathcal I}\sqrt{Q^{(1)}_{p,a}}.
  \label{eq:appendix-direct-energy-bound}
\end{equation}
The interval computation certifies
\[
  \sum_{(p,a)\in\mathcal I}\sqrt{Q^{(0)}_{p,a}}
  \le9.18605826,
  \qquad
  \sum_{(p,a)\in\mathcal I}\sqrt{Q^{(1)}_{p,a}}
  \le20.73000771.
\]
Substitution into \eqref{eq:appendix-direct-energy-bound} yields
\begin{equation}
  \|D^3H\|_{L^2(\mathbb T)}
  \le9.18605826+\frac{\pi}{\sqrt6}(20.73000771)
  <35.773327<35.774.
  \label{eq:appendix-energy-output}
\end{equation}
Together, \eqref{eq:appendix-head-output} and
\eqref{eq:appendix-energy-output} prove
Proposition~\ref{prop:certified-numerical-input}.

\subsection{Interval-arithmetic implementation}
\label{app:certification-implementation}

For reproducibility, the implementation records the following data.

\begin{enumerate}
  \item Every decimal parameter is treated as an exact terminating rational,
  or is replaced by an explicit outward-rounded interval.
  \item The one-dimensional coefficient integrals are evaluated by adaptive
  interval quadrature on a finite interval, with a closed Gaussian-tail bound
  outside that interval.
  \item Every derivative of $K_r$ is reduced to a polynomially weighted
  Gaussian integral.  The mixed exponential is expanded into an absolutely
  convergent series with a certified tail.
  \item The circle averages are enclosed by a composite four-point
  Gauss--Legendre rule.  A panelwise eighth-derivative estimate supplies the
  rigorous remainder; the computation uses $2048$ panels.
  \item On every panel, the code verifies that $1-\rho(e^{i\theta})^2$ avoids
  zero and that the Gaussian decay margin remains positive.  This also gives
  the domination needed for the radial boundary passage above.
\end{enumerate}

The certificate terminates by printing the outward-rounded statements
\[
  b_1\ge0.881573822049,
  \qquad
  \sum_{\substack{3\le m\le251\\m\ \mathrm{odd}}}|b_m|
  \le1.1328860\cdot10^{-5},
  \qquad
  \|D^3H\|_{L^2(\mathbb T)}<35.774,
\]
and
\[
  0.881545409+1.1328860\cdot10^{-5}
  +\frac{36}{\sqrt{10\cdot251^5}}
  <0.881573822049.
\]
The last inequality is the complete numerical bridge from this appendix to
Section~\ref{sec:certification}.
