# Supplementary material for: Long-Horizon AI Research for Grothendieck Constant: A Case Study in Human-AI Mathematical Collaboration
Source: arXiv:2608.11195 source file (2026-08-14)
Supplement: Supplementary file 4 [file appendix.tex]

\newpage
\appendix

\section{Krivine Preprocessing and Mixed Rounding}
\label[appendix]{app:krivine-preprocessing}

This appendix records the preprocessing and projection arguments behind
Krivine rounding schemes.
The argument is the standard rounding construction
~\cite{krivine1977constante, braverman2011grothendieckconstantstrictlysmaller}.

For a real matrix \(A=(a_{ij})\in\mathbb R^{m\times n}\), write
\[
    \operatorname{SDP}(A)
    :=
    \sup_{\|x_i\|=\|y_j\|=1}
    \left|
        \sum_{i=1}^m\sum_{j=1}^n a_{ij}\langle x_i,y_j\rangle
    \right|
\]
and
\[
    \operatorname{OPT}(A)
    :=
    \max_{\varepsilon_i,\delta_j\in\{\pm 1\}}
    \left|
        \sum_{i=1}^m\sum_{j=1}^n a_{ij}\varepsilon_i\delta_j
    \right|.
\]
Thus proving \(\operatorname{SDP}(A)\le K\operatorname{OPT}(A)\) for all
\(A\) proves \(K_G\le K\).

\begin{theorem}[Krivine preprocessing and projection]
\label{thm:appendix-pure-krivine-rounding}
Let \(f,g:\mathbb R^k\to\{-1,1\}\) be odd measurable functions, and let
\(H=H_{f,g}\) be the arcsine-normalized correlation function
\[
    H(t)
    =
    \frac{\pi}{2}
    \mathbb E\left[
        f\left(G_1\right)
        g\left(tG_1+\sqrt{1-t^2}G_2\right)
    \right],
    \qquad -1<t<1,
\]
where \(G_1,G_2\) are independent standard Gaussian vectors in
\(\mathbb R^k\). Suppose that \(H\) has a local inverse at the origin,
\[
    H^{-1}(\zeta)=\sum_{r\ge 1} a_r\zeta^r,
\]
which is holomorphic on a neighborhood of \(\gamma\overline{\mathbb D}\),
and suppose that
\[
    \sum_{r\ge 1}|a_r|\gamma^r\le 1.
\]
Then
\[
    K_G\le \frac{\pi}{2\gamma}.
\]
\end{theorem}

\begin{proof}
It is enough to prove the conclusion with any \(0<\gamma'<\gamma\) in
place of \(\gamma\), and then let \(\gamma'\uparrow\gamma\). We therefore
fix such a \(\gamma'\). Put
\[
    M_{\gamma'}:=\sum_{r\ge 1}|a_r|(\gamma')^r < 1.
\]
Let \(A=(a_{ij})\in\mathbb R^{m\times n}\). Choose unit vectors
\(x_1,\ldots,x_m,y_1,\ldots,y_n\) such that
\[
    \sum_{i,j} a_{ij}\langle x_i,y_j\rangle
\]
is arbitrarily close to \(\operatorname{SDP}(A)\); if necessary, replace all
\(y_j\) by \(-y_j\) so that this quantity is nonnegative. We suppress this
arbitrarily small error, since it disappears at the end.

Let
\[
    \mathcal K
    :=
    \left(\bigoplus_{r\ge 1} \mathcal H^{\otimes r}\right)
    \oplus \mathbb R e_L\oplus \mathbb R e_R,
\]
where \(\mathcal H\) is the Hilbert space containing the original vectors,
and where \(e_L,e_R\) are unit vectors orthogonal to each other and to all
tensor summands. Define
\[
    I(x)
    :=
    \bigoplus_{r\ge 1}
        \sqrt{|a_r|}\,(\gamma')^{r/2}x^{\otimes r}
    \oplus \sqrt{1-M_{\gamma'}}\,e_L
    \oplus 0
\]
and
\[
    J(y)
    :=
    \bigoplus_{r\ge 1}
        \operatorname{sgn}(a_r)\sqrt{|a_r|}\,(\gamma')^{r/2}y^{\otimes r}
    \oplus 0
    \oplus \sqrt{1-M_{\gamma'}}\,e_R,
\]
with the convention that the summand corresponding to \(a_r=0\) is zero.
Then \(I(x)\) and \(J(y)\) are unit vectors whenever \(x,y\) are unit
vectors. Moreover,
\[
    \langle I(x),J(y)\rangle
    =
    \sum_{r\ge 1} a_r(\gamma')^r\langle x,y\rangle^r
    =
    H^{-1}\bigl(\gamma'\langle x,y\rangle\bigr).
\]
The first equality uses
\[
    \langle x^{\otimes r},y^{\otimes r}\rangle
    =
    \langle x,y\rangle^r,
\]
and the second equality uses the Taylor expansion of the inverse on
\(\gamma'\mathbb D\).

Set
\[
    u_i:=I(x_i),
    \qquad
    v_j:=J(y_j).
\]
The finitely many vectors \(u_i,v_j\) span a finite-dimensional subspace of
\(\mathcal K\). Identify this subspace with \(\mathbb R^N\). Let
\(\Gamma:\mathbb R^N\to\mathbb R^k\) be a random Gaussian linear map, i.e.
a \(k\times N\) matrix whose entries are independent standard Gaussian
random variables. Define random signs
\[
    \varepsilon_i
    :=
    f\left(\Gamma u_i\right),
    \qquad
    \delta_j
    :=
    g\left(\Gamma v_j\right).
\]
For each pair \((i,j)\), the vectors \(\Gamma u_i\) and \(\Gamma v_j\) are
standard Gaussian vectors in \(\mathbb R^k\) with coordinatewise correlation
\(\langle u_i,v_j\rangle\). Hence, by the definition of \(H\),
\[
    \mathbb E[\varepsilon_i\delta_j]
    =
    \frac{2}{\pi}
    H(\langle u_i,v_j\rangle).
\]
Using the preprocessing identity,
\[
    H(\langle u_i,v_j\rangle)
    =
    H\left(H^{-1}\bigl(\gamma'\langle x_i,y_j\rangle\bigr)\right)
    =
    \gamma'\langle x_i,y_j\rangle.
\]
Therefore
\[
\begin{aligned}
    \mathbb E\left[\sum_{i,j} a_{ij}\varepsilon_i\delta_j\right]
    &=
    \frac{2}{\pi}\sum_{i,j}a_{ij}
        H(\langle u_i,v_j\rangle) \\
    &=
    \frac{2\gamma'}{\pi}
    \sum_{i,j}a_{ij}\langle x_i,y_j\rangle.
\end{aligned}
\]
Since the maximum over deterministic signs is at least the expectation of
the randomized signs, we get
\[
    \operatorname{OPT}(A)
    \ge
    \frac{2\gamma'}{\pi}\operatorname{SDP}(A).
\]
Thus
\[
    \operatorname{SDP}(A)
    \le
    \frac{\pi}{2\gamma'}\operatorname{OPT}(A).
\]
Letting \(\gamma'\uparrow\gamma\) gives
\[
    \operatorname{SDP}(A)
    \le
    \frac{\pi}{2\gamma}\operatorname{OPT}(A).
\]
Since \(A\) was arbitrary, \(K_G\le \pi/(2\gamma)\).
\end{proof}

\begin{corollary}[Classical Krivine hyperplane bound]
\label{cor:appendix-classical-krivine}
Let \(h:\mathbb R\to\{-1,1\}\) be \(h(x)=\operatorname{sgn}(x)\). Then the
hyperplane scheme \((h,h)\) gives
\[
    K_G\le \frac{\pi}{2\log(1+\sqrt 2)}.
\]
\end{corollary}

\begin{proof}
For the hyperplane scheme, Grothendieck's identity gives
\[
    \mathbb E[\operatorname{sgn}(X)\operatorname{sgn}(Y)]
    =
    \frac{2}{\pi}\arcsin(t)
\]
whenever \(X,Y\) are standard Gaussians with correlation \(t\). In our
normalization,
\[
    H_{h,h}(t)=\arcsin(t).
\]
Thus
\[
    H_{h,h}^{-1}(\zeta)=\sin \zeta
    =
    \sum_{q\ge 0}\frac{(-1)^q}{(2q+1)!}\zeta^{2q+1}.
\]
Let
\[
    \rho_*:=\operatorname{arsinh}(1)=\log(1+\sqrt 2).
\]
Then
\[
    \sum_{q\ge 0}
    \frac{\rho_*^{2q+1}}{(2q+1)!}
    =
    \sinh(\rho_*)
    =
    1.
\]
Theorem~\ref{thm:appendix-pure-krivine-rounding} therefore applies with
\(\gamma=\rho_*\), giving
\[
    K_G\le \frac{\pi}{2\rho_*}
    =
    \frac{\pi}{2\log(1+\sqrt 2)}.
\]
\end{proof}

\begin{theorem}[Mixed Krivine preprocessing and projection]
\label{thm:appendix-mixed-krivine-rounding}
Let \(L\in\mathbb N\). For each \(\ell\in\{1,\ldots,L\}\), let
\(f_\ell,g_\ell:\mathbb R^{k_\ell}\to\{-1,1\}\) be odd measurable functions,
and let \(H_\ell\) be the corresponding arcsine-normalized correlation
function:
\[
    H_\ell(t)
    =
    \frac{\pi}{2}
    \mathbb E\left[
        f_\ell\left(G_1\right)
        g_\ell\left(tG_1+\sqrt{1-t^2}G_2\right)
    \right].
\]
Let \(\lambda_1,\ldots,\lambda_L\ge 0\) satisfy
\(\sum_{\ell=1}^L\lambda_\ell=1\), and define the mixed function
\[
    H_\lambda(t):=\sum_{\ell=1}^L\lambda_\ell H_\ell(t).
\]
Suppose that \(H_\lambda\) has a local inverse at the origin,
\[
    H_\lambda^{-1}(\zeta)=\sum_{r\ge 1} a_r\zeta^r,
\]
which is holomorphic on a neighborhood of \(\gamma\overline{\mathbb D}\),
and suppose that
\[
    M_\lambda(\gamma)
    :=
    \sum_{r\ge 1}|a_r|\gamma^r
    \le 1.
\]
Then
\[
    K_G\le \frac{\pi}{2\gamma}.
\]
\end{theorem}

\begin{proof}
The preprocessing is identical to the proof of
Theorem~\ref{thm:appendix-pure-krivine-rounding}, but using the inverse
coefficients of \(H_\lambda^{-1}\). As before, first fix
\(0<\gamma'<\gamma\), and set
\[
    M_{\lambda,\gamma'}
    :=
    \sum_{r\ge 1}|a_r|(\gamma')^r
    <1.
\]
For unit vectors \(x,y\), define
\[
    I(x)
    :=
    \bigoplus_{r\ge 1}
        \sqrt{|a_r|}\,(\gamma')^{r/2}x^{\otimes r}
    \oplus \sqrt{1-M_{\lambda,\gamma'}}\,e_L
    \oplus 0
\]
and
\[
    J(y)
    :=
    \bigoplus_{r\ge 1}
        \operatorname{sgn}(a_r)\sqrt{|a_r|}\,(\gamma')^{r/2}y^{\otimes r}
    \oplus 0
    \oplus \sqrt{1-M_{\lambda,\gamma'}}\,e_R.
\]
Then \(I(x)\) and \(J(y)\) are unit vectors and
\[
    \langle I(x),J(y)\rangle
    =
    H_\lambda^{-1}\bigl(\gamma'\langle x,y\rangle\bigr).
\]

Now let \(A=(a_{ij})\) be arbitrary, and choose unit vectors
\(x_i,y_j\) that nearly attain \(\operatorname{SDP}(A)\), oriented so that
\(\sum_{i,j}a_{ij}\langle x_i,y_j\rangle\ge 0\). Put
\[
    u_i:=I(x_i),
    \qquad
    v_j:=J(y_j).
\]
Identify the span of the finitely many \(u_i,v_j\) with \(\mathbb R^N\).
For each \(\ell\), independently sample a Gaussian linear map
\[
    \Gamma_\ell:\mathbb R^N\to\mathbb R^{k_\ell}.
\]
Also sample a single global index \(\Lambda\in\{1,\ldots,L\}\), independent
of the Gaussian maps, with
\[
    \mathbb P[\Lambda=\ell]=\lambda_\ell.
\]
The word ``global'' is important: the same index \(\Lambda\) is used for
all \(i,j\). Define
\[
    \varepsilon_i
    :=
    f_\Lambda\left(\Gamma_\Lambda u_i\right),
    \qquad
    \delta_j
    :=
    g_\Lambda\left(\Gamma_\Lambda v_j\right).
\]
Conditioning on \(\Lambda=\ell\), the same rotation-invariance calculation
as in the pure case gives
\[
    \mathbb E[\varepsilon_i\delta_j\mid \Lambda=\ell]
    =
    \frac{2}{\pi}H_\ell(\langle u_i,v_j\rangle).
\]
Averaging over \(\Lambda\),
\[
    \mathbb E[\varepsilon_i\delta_j]
    =
    \frac{2}{\pi}
    \sum_{\ell=1}^L\lambda_\ell H_\ell(\langle u_i,v_j\rangle)
    =
    \frac{2}{\pi}H_\lambda(\langle u_i,v_j\rangle).
\]
Since
\[
    \langle u_i,v_j\rangle
    =
    H_\lambda^{-1}\bigl(\gamma'\langle x_i,y_j\rangle\bigr),
\]
we obtain
\[
    \mathbb E[\varepsilon_i\delta_j]
    =
    \frac{2\gamma'}{\pi}\langle x_i,y_j\rangle.
\]
Therefore
\[
\begin{aligned}
    \operatorname{OPT}(A)
    &\ge
    \mathbb E\left[
        \sum_{i,j}a_{ij}\varepsilon_i\delta_j
    \right] \\
    &=
    \frac{2\gamma'}{\pi}
    \sum_{i,j}a_{ij}\langle x_i,y_j\rangle.
\end{aligned}
\]
Taking the supremum over the original vectors gives
\[
    \operatorname{OPT}(A)
    \ge
    \frac{2\gamma'}{\pi}\operatorname{SDP}(A),
\]
and hence
\[
    \operatorname{SDP}(A)
    \le
    \frac{\pi}{2\gamma'}\operatorname{OPT}(A).
\]
Letting \(\gamma'\uparrow\gamma\) proves
\[
    \operatorname{SDP}(A)
    \le
    \frac{\pi}{2\gamma}\operatorname{OPT}(A).
\]
Since \(A\) was arbitrary, \(K_G\le \pi/(2\gamma)\).
\end{proof}

\begin{remark}
Theorem~\ref{thm:appendix-pure-krivine-rounding} is the special case
\(L=1\) of Theorem~\ref{thm:appendix-mixed-krivine-rounding}. We separated
the two statements because the pure case is the usual Krivine scheme, while
the mixed case emphasizes the randomized choice of a common scheme
\(\Lambda\) before projection.
\end{remark}


\section{General Coefficient Formulas}
\label{app:coefficient-formulas}

This appendix records two standard calculations used in
Section~\ref{sec:coefficients}. We first prove the closed form for the
one-dimensional threshold coefficients. We then give the coefficient
formula for a more general limiting scheme built from several Hermite
correlation coordinates. The latter is not needed for the main theorem,
but it explains how the calculation extends to other odd degrees.

\begin{lemma}[One-dimensional threshold coefficients]
\label{lem:qk}
Let \(Z\) be a standard Gaussian and define
\(
q_k(u)=\E[\sgn(Z+u)\He_k(Z)]
\).
Then
\[
    q_0(u)
    =
    \erf\left(\frac{u}{\sqrt{2}}\right),
\]
and, for \(k\geq 1\),
\[
    q_k(u)
    =
    \frac{2\varphi(u)}{\sqrt{k}}\He_{k-1}(-u),
\]
where \(\varphi(u)=(2\pi)^{-1/2}e^{-u^2/2}\).
\end{lemma}

\begin{proof}
The formula for \(q_0\) follows directly from the Gaussian distribution
function. For \(k\geq 1\), orthogonality to constants gives
\[
    q_k(u)
    =
    2\int_{-u}^{\infty}\He_k(z)\varphi(z)\,dz.
\]
The orthonormal probabilists' Hermite polynomials satisfy
\[
    \frac{d}{dz}
    \bigl(\varphi(z)\He_{k-1}(z)\bigr)
    =
    -\sqrt{k}\,\varphi(z)\He_k(z).
\]
Integrating from \(-u\) to \(\infty\) proves the claim.
\end{proof}

We next record the general formula. Let \(D\) be a finite set of odd
integers. Fix weights \((s_d)_{d\in D}\), set
\[
    S
    =
    \left(\sum_{d\in D}s_d^2\right)^{1/2},
    \qquad
    \alpha_d
    =
    \frac{s_d}{S},
\]
and let \(\sigma_d\in\{-1,1\}\). Consider the limiting Krivine scheme
with partitions
\[
    f_D(z,x,(r_d)_{d\in D})
    =
    \sgn\!\left(
        z+\eta\He_3(x)+\sum_{d\in D}s_dr_d
    \right),
\]
\[
    g_D(z,x,(r_d)_{d\in D})
    =
    \sgn\!\left(
        z-\eta\He_3(x)+\sum_{d\in D}\sigma_ds_dr_d
    \right),
\]
whose coordinate correlation maps are \(t,t\), and \(t^d\) for
\(d\in D\).

For \(a,b,k\geq 0\), define
\begin{equation}
    C_{a,b,k}
    =
    \E\!\left[
        \He_a(Z)\He_b(X)
        q_k\!\left(
            \frac{Z+\eta\He_3(X)}{S}
        \right)
    \right],
    \label{eq:general-Cabk}
\end{equation}
where \(Z,X\) are independent standard Gaussians. For a multi-index
\(\nu=(\nu_d)_{d\in D}\), write
\(
|\nu|=\sum_d\nu_d
\),
\(
\nu!=\prod_d\nu_d!
\), and
\(
\alpha^\nu=\prod_d\alpha_d^{\nu_d}
\).

\begin{proposition}[General degree formula]
\label{prop:general-degree-formula}
Let
\(
H_D(t)=\sum_{m\geq 1}b_m t^m
\)
be the correlation function of the scheme above. Then
\begin{equation}
    b_m
    =
    \frac{\pi}{2}
    \sum_{\substack{a,b\geq 0,\ \nu\in\mathbb{N}_0^D\\
          a+b+\sum_{d\in D}d\nu_d=m}}
    (-1)^b
    \left(\prod_{d\in D}\sigma_d^{\nu_d}\right)
    \frac{k!}{\nu!}
    \left(\prod_{d\in D}\alpha_d^{2\nu_d}\right)
    C_{a,b,k}^2,
    \qquad
    k=|\nu|.
    \label{eq:general-bm-appendix}
\end{equation}
Only odd \(m\) occur.
\end{proposition}

\begin{proof}
Set
\[
    T(Z,X)=Z+\eta\He_3(X),
    \qquad
    R_\alpha=\sum_{d\in D}\alpha_dR_d.
\]
Then \(f_D=\sgn(T+SR_\alpha)\). Conditioning on \(Z,X\), the coefficient
of \(\He_k(R_\alpha)\) is
\(
q_k(T(Z,X)/S)
\). Taking the inner product with
\(\He_a(Z)\He_b(X)\) gives \(C_{a,b,k}\).

The multivariate Hermite addition formula is
\[
    \He_k\!\left(\sum_{d\in D}\alpha_dR_d\right)
    =
    \sum_{\substack{\nu\in\mathbb{N}_0^D\\|\nu|=k}}
    \sqrt{\frac{k!}{\nu!}}\,
    \alpha^\nu
    \prod_{d\in D}\He_{\nu_d}(R_d).
\]
Hence the coefficient of
\(
\He_a(Z)\He_b(X)\prod_d\He_{\nu_d}(R_d)
\)
in \(f_D\) is
\[
    C_{a,b,k}
    \sqrt{\frac{k!}{\nu!}}\,
    \alpha^\nu.
\]
The corresponding coefficient of \(g_D\) differs by the factor
\(
(-1)^b\prod_d\sigma_d^{\nu_d}
\).

Under the limiting scheme, the matching Hermite term contributes
\[
    t^a t^b\prod_{d\in D}(t^d)^{\nu_d}
    =
    t^{a+b+\sum_d d\nu_d}.
\]
Multiplying the two Hermite coefficients and collecting the coefficient
of \(t^m\) gives \eqref{eq:general-bm-appendix}. Finally, both partitions
are odd, so their Hermite coefficients vanish unless
\(a+b+|\nu|\) is odd. Since every \(d\in D\) is odd, this has the same
parity as \(a+b+\sum_d d\nu_d\).
\end{proof}


% Insert this section after \appendix in paper/appendix.tex.
\section{Certification Details}
\label{app:certification-details}

This appendix proves Proposition~\ref{prop:certified-numerical-input}.  The
first computation encloses the coefficient head through degree $251$.  The
second bounds the single boundary norm
$\|D^3H\|_{L^2(\mathbb T)}$ used in
Lemma~\ref{lem:third-order-tail}.

\subsection{The coefficient head}
\label{app:certification-coefficient-head}

Let $W,X$ be independent standard Gaussians and write
\[
  f(w,x)=\operatorname{sgn}\bigl(w+\vartheta\operatorname{He}_3(x)\bigr).
\]
For $a,b\ge0$, define
\[
  A_{a,b}
  :=\mathbb E\bigl[f(W,X)\operatorname{He}_a(W)
  \operatorname{He}_b(X)\bigr].
\]
As shown in Section~4, if
\[
  \rho(t)=\frac{t-s_3^2t^3+s_5^2t^5}{1+s_3^2+s_5^2},
\]
then
\begin{equation}
  H(t)=\frac{\pi}{2}\sum_{a,b\ge0}A_{a,b}^2\rho(t)^a(-t)^b,
  \label{eq:appendix-correlation-expansion}
\end{equation}
and hence
\begin{equation}
  b_m=\frac{\pi}{2}
  \sum_{\substack{a,b\ge0\\a+b\le m}}
  (-1)^bA_{a,b}^2[t^{m-b}]\rho(t)^a.
  \label{eq:appendix-coefficient-formula}
\end{equation}

The coefficients $A_{a,b}$ reduce to one-dimensional Gaussian integrals.  If
$Z$ is standard Gaussian and
\[
  q_a(u):=\mathbb E[\operatorname{sgn}(Z+u)\operatorname{He}_a(Z)],
\]
then
\[
  A_{a,b}
  =\mathbb E\bigl[\operatorname{He}_b(X)
  q_a(\vartheta\operatorname{He}_3(X))\bigr],
\]
where
\[
  q_0(u)=\operatorname{erf}\!\left(\frac{u}{\sqrt2}\right),
  \qquad
  q_a(u)=\frac{2\varphi(u)}{\sqrt a}
  \operatorname{He}_{a-1}(-u)
  \quad(a\ge1).
\]
Each integral is enclosed by outward-rounded adaptive quadrature on a finite
interval, together with a closed Gaussian-tail estimate.  Finite coefficient
extraction in \eqref{eq:appendix-coefficient-formula} then gives
\begin{equation}
  b_1\ge0.881573822049,
  \qquad
  \sum_{\substack{3\le m\le251\\m\ \mathrm{odd}}}|b_m|
  \le1.1328860\cdot10^{-5}.
  \label{eq:appendix-head-output}
\end{equation}

\subsection{A boundary representation of $D^3H$}
\label{app:certification-boundary-representation}

For real $|r|<1$, let
\[
  K_r(u,v)
  :=\frac{1}{2\pi\sqrt{1-r^2}}
  \exp\!\left(-\frac{u^2-2ruv+v^2}{2(1-r^2)}\right)
\]
be the centered bivariate Gaussian density with correlation $r$.  Let
$C_r(x,y)$ denote the conditional sign-correlation kernel
\[
  C_r(x,y)
  :=\frac{\pi}{2}\,
  \mathbb E\!\left[
  \operatorname{sgn}(W+\vartheta\operatorname{He}_3(x))
  \operatorname{sgn}(W'+\vartheta\operatorname{He}_3(y))
  \right],
\]
where $(W,W')$ is a standard Gaussian pair with correlation $r$.
The two derivative identities needed below follow directly from the Hermite
expansion of this kernel.

\begin{lemma}[Differentiating the threshold-correlation kernel]
\label{lem:appendix-kernel-differentiation}
For real $|r|<1$,
\begin{align}
  \partial_rC_r(x,y)
  &=2\pi K_r\bigl(\vartheta\operatorname{He}_3(x),
                   \vartheta\operatorname{He}_3(y)\bigr),
  \label{eq:appendix-kernel-r}\\
  \partial_x\partial_yC_r(x,y)
  &=2\pi\vartheta^2\operatorname{He}_3'(x)
  \operatorname{He}_3'(y)
  K_r\bigl(\vartheta\operatorname{He}_3(x),
           \vartheta\operatorname{He}_3(y)\bigr).
  \label{eq:appendix-kernel-xy}
\end{align}
\end{lemma}

\begin{proof}
Put
\[
  u=\vartheta\operatorname{He}_3(x),
  \qquad
  v=\vartheta\operatorname{He}_3(y).
\]
The Hermite covariance identity gives
\begin{equation}
  C_r(x,y)=\frac{\pi}{2}\sum_{a\ge0}r^a q_a(u)q_a(v),
  \label{eq:appendix-Cr-Hermite}
\end{equation}
where $q_a$ is the one-dimensional threshold coefficient defined above.  The
series and its $r$-derivative converge locally uniformly for $|r|<1$.  For
$a\ge1$,
\[
  q_a(u)=\frac{2\varphi(u)}{\sqrt a}\operatorname{He}_{a-1}(-u).
\]
Consequently,
\begin{align*}
  \partial_rC_r(x,y)
  &=\frac{\pi}{2}\sum_{a\ge1}a r^{a-1}q_a(u)q_a(v)\\
  &=2\pi\varphi(u)\varphi(v)
    \sum_{n\ge0}r^n\operatorname{He}_n(-u)
                         \operatorname{He}_n(-v).
\end{align*}
Mehler's identity identifies the last expression with $2\pi K_r(u,v)$,
proving \eqref{eq:appendix-kernel-r}.

Differentiating the defining integral for $q_a$ gives, for every $a\ge0$,
\[
  q_a'(u)=2\varphi(u)\operatorname{He}_a(-u).
\]
Differentiating \eqref{eq:appendix-Cr-Hermite} in $x$ and $y$ and applying
Mehler's identity once more yields
\begin{align*}
  \partial_x\partial_yC_r(x,y)
  &=\frac{\pi}{2}\vartheta^2\operatorname{He}_3'(x)
    \operatorname{He}_3'(y)
    \sum_{a\ge0}r^a q_a'(u)q_a'(v)\\
  &=2\pi\vartheta^2\operatorname{He}_3'(x)
    \operatorname{He}_3'(y)K_r(u,v),
\end{align*}
which proves \eqref{eq:appendix-kernel-xy}.
\end{proof}

Thus, after one derivative, the discontinuous sign functions are replaced by
explicit smooth Gaussian kernels.  The formulas above initially hold for
$|r|<1$; the explicit Gaussian expressions provide the analytic continuation
used on the complex curve $r=\rho(e^{i\theta})$ below.

If $\Psi$ has Hermite coefficients $\widehat\Psi_{i,j}$, define the diagonal
trace
\[
  T_\lambda[\Psi]
  :=\widehat\Psi_{0,0}+\sum_{n\ge1}\lambda^n\widehat\Psi_{n,n},
  \qquad |\lambda|\le1.
\]
For $|\lambda|<1$, this is the expectation of $\Psi(X,Y)$ when $(X,Y)$ is a
standard Gaussian pair with correlation $\lambda$.

\begin{lemma}[Differentiating the diagonal trace]
\label{lem:appendix-trace-differentiation}
If $\Psi(t)$ is a sufficiently regular family of kernels, then for $|t|<1$,
\begin{equation}
  D_tT_{-t}[\Psi(t)]
  =T_{-t}\!\left[D_t\Psi(t)-t\partial_x\partial_y\Psi(t)\right],
  \qquad D_t=t\partial_t.
  \label{eq:appendix-trace-differentiation}
\end{equation}
\end{lemma}

\begin{proof}
Write
\[
  \Psi(t;x,y)=\sum_{i,j\ge0}\widehat\Psi_{i,j}(t)
  \operatorname{He}_i(x)\operatorname{He}_j(y).
\]
Since $D_t(-t)^n=n(-t)^n$, termwise differentiation gives
\[
  D_tT_{-t}[\Psi(t)]
  =T_{-t}[D_t\Psi(t)]
   +\sum_{n\ge1}n(-t)^n\widehat\Psi_{n,n}(t).
\]
The identity
$\frac{d}{dx}\operatorname{He}_n(x)=\sqrt n\operatorname{He}_{n-1}(x)$
shows that
\[
  -tT_{-t}[\partial_x\partial_y\Psi(t)]
  =\sum_{n\ge1}n(-t)^n\widehat\Psi_{n,n}(t).
\]
Combining the last two displays proves
\eqref{eq:appendix-trace-differentiation}.
\end{proof}

The Cauchy--Schwarz inequality gives the boundary trace estimate
\begin{equation}
  |T_\lambda[\Psi]|
  \le
  \|\Psi\|_{L^2(\mu)}
  +\frac{\pi}{\sqrt6}
  \|\partial_x\partial_y\Psi\|_{L^2(\mu)},
  \label{eq:appendix-trace-bound}
\end{equation}
where $\mu$ is product standard Gaussian measure.

For $|t|<1$, one has
\[
  H(t)=T_{-t}[C_{\rho(t)}].
\]
Define
\[
  \Phi_0(t;x,y):=C_{\rho(t)}(x,y),
  \qquad
  \Phi_{k+1}:=D_t\Phi_k-t\partial_x\partial_y\Phi_k.
\]
Applying the differentiation identity three times gives
\begin{equation}
  D^3H(t)=T_{-t}[\Phi_3(t;\cdot,\cdot)].
  \label{eq:appendix-D3-trace}
\end{equation}
The interval bounds below provide a uniform integrable majorant, which
justifies taking radial limits in \eqref{eq:appendix-D3-trace} as
$|t|\uparrow1$.

\subsection{The nine smooth kernels}
\label{app:certification-nine-kernels}

Write $\rho_j=D_t^j\rho$.  For $p+a\ge1$, set
\[
  G_{p,a}(t;x,y)
  :=\left[
  \partial_r^p(\partial_x\partial_y)^aC_r(x,y)
  \right]_{r=\rho(t)}.
\]
Expanding the recursion before taking norms gives
\[
  \Phi_3(t;x,y)
  =\sum_{(p,a)\in\mathcal I}c_{p,a}(t)G_{p,a}(t;x,y),
\]
where
\[
  \mathcal I=
  \{(1,0),(2,0),(3,0),(0,1),(0,2),(0,3),
    (1,1),(2,1),(1,2)\},
\]
and
\begin{center}
\begin{tabular}{c c@{\qquad}c c}
\toprule
$(p,a)$ & $c_{p,a}(t)$ & $(p,a)$ & $c_{p,a}(t)$\\
\midrule
$(1,0)$ & $\rho_3$ & $(0,1)$ & $-t$\\
$(2,0)$ & $3\rho_1\rho_2$ & $(0,2)$ & $3t^2$\\
$(3,0)$ & $\rho_1^3$ & $(0,3)$ & $-t^3$\\
$(1,1)$ & $-3t(\rho_1+\rho_2)$ & $(2,1)$ & $-3t\rho_1^2$\\
$(1,2)$ & $3t^2\rho_1$ & & \\
\bottomrule
\end{tabular}
\end{center}

For $t=e^{i\theta}$ on the unit circle, define the combined energy
\[
  S(\theta)
  :=\bigl\|\Phi_3(e^{i\theta})\bigr\|_{L^2(\mu)}^2
  +4\,\bigl\|\partial_x\partial_y\Phi_3(e^{i\theta})\bigr\|_{L^2(\mu)}^2.
\]
By \eqref{eq:appendix-D3-trace}, the trace estimate
\eqref{eq:appendix-trace-bound}, and the Cauchy--Schwarz inequality
\[
  \Bigl(x+\tfrac{\pi}{\sqrt6}\,y\Bigr)^2
  \le\Bigl(1+\tfrac{\pi^2}{24}\Bigr)\bigl(x^2+4y^2\bigr)
  \le\tfrac{\pi^2}{6}\bigl(x^2+4y^2\bigr),
\]
one has the pointwise bound
$|D^3H(e^{i\theta})|^2\le\tfrac{\pi^2}{6}S(\theta)$.  Since every
construction coefficient is real, $S(-\theta)=S(\theta)$, and therefore
\begin{equation}
  \|D^3H\|_{L^2(\mathbb T)}^2
  =\frac{1}{2\pi}\int_0^{2\pi}
  \bigl|D^3H(e^{i\theta})\bigr|^2\,d\theta
  \le\frac{\pi^2}{6}\cdot\frac{1}{\pi}\int_0^{\pi}S(\theta)\,d\theta.
  \label{eq:appendix-combined-energy}
\end{equation}
The interval computation certifies
\[
  \frac{1}{\pi}\int_0^{\pi}S(\theta)\,d\theta
  \le126.80385221.
\]
Substitution into \eqref{eq:appendix-combined-energy} yields
\begin{equation}
  \|D^3H\|_{L^2(\mathbb T)}
  \le\frac{\pi}{\sqrt6}\,\bigl(126.80385221\bigr)^{1/2}
  <14.443.
  \label{eq:appendix-energy-output}
\end{equation}
Together, \eqref{eq:appendix-head-output} and
\eqref{eq:appendix-energy-output} prove
Proposition~\ref{prop:certified-numerical-input}.

\subsection{Interval-arithmetic implementation}
\label{app:certification-implementation}

For reproducibility, the implementation records the following data.

\begin{enumerate}
  \item Every decimal parameter is treated as an exact terminating rational,
  or is replaced by an explicit outward-rounded interval.
  \item The one-dimensional coefficient integrals are evaluated by adaptive
  interval quadrature on a finite interval, with a closed Gaussian-tail bound
  outside that interval.
  \item Every derivative of $K_r$ is reduced to a polynomially weighted
  Gaussian integral.  The mixed exponential is expanded into an absolutely
  convergent series with a certified tail.
  \item The circle average of $S$ is enclosed by a composite four-point
  Gauss--Legendre rule.  A panelwise eighth-derivative estimate supplies the
  rigorous remainder; by the symmetry $S(-\theta)=S(\theta)$ the average is
  taken over $[0,\pi]$, and the computation uses $1024$ panels.
  \item On every panel, the code verifies the uniform bounds
  $\lvert1-\rho(e^{i\theta})^2\rvert\ge0.3724$ and a Gaussian decay margin of
  at least $0.49$.  This also gives the domination needed for the radial
  boundary passage above.
\end{enumerate}

The certificate terminates by printing the outward-rounded statements
\[
  b_1\ge0.881573822049,
  \qquad
  \sum_{\substack{3\le m\le251\\m\ \mathrm{odd}}}|b_m|
  \le1.1328860\cdot10^{-5},
  \qquad
  \|D^3H\|_{L^2(\mathbb T)}<14.443,
\]
and
\[
  0.881545409+1.1328860\cdot10^{-5}
  +\frac{14.443}{\sqrt{10\cdot251^5}}
  <0.881573822049.
\]
The last inequality is the complete numerical bridge from this appendix to
Section~\ref{sec:certification}.







% \section{Proof of rearrangement lemma}
% \label{app:rearrangement_lemma}

% \begin{lemma}[One-dimensional rearrangement]
% Let $S\sim N(0,1)$ and $x\in[0,1]$. Then
% \[
%         \sup_{\substack{|A|\le1\\ \E[A(S)S]=\nu x}}
%         \E[A(S)(S^3-3S)]
%         =-\nu\Delta(x).
% \]
% \end{lemma}

% \begin{proof}
% Fix $r\ge0$ by
% \[
%         e^{-r^2/2}=\frac{1+x}{2},
% \]
% and put
% \[
%         \mu=r^2-3.
% \]
% Let $W=S^3-3S$. Then
% \[
%         W-\mu S=S^3-3S-(r^2-3)S=S(S^2-r^2).
% \]

% For any feasible $A$,
% \begin{align*}
%         \E[AW]
%         &=\E[A(W-\mu S)]+\mu\E[AS]\\
%         &=\E[A(W-\mu S)]+\mu\nu x\\
%         &\le \E|W-\mu S|+\mu\nu x,
% \end{align*}
% using $|A|\le1$.

% Equality is attained by
% \[
%         A_*(S)=\sgn(W-\mu S)=\sgn(S)\sgn(S^2-r^2),
% \]
% provided $A_*$ has the right first moment. It does, because
% \[
%         A_*(S)S=|S|\sgn(S^2-r^2),
% \]
% so
% \begin{align*}
%         \E[A_*(S)S]
%         &=2\E[|S|\one_{|S|>r}]-\E|S|\\
%         &=2\nu e^{-r^2/2}-\nu\\
%         &=\nu x.
% \end{align*}
% Thus $A_*$ is feasible and attains the dual upper bound.

% It remains to compute its value. Since
% \[
%         \sgn(S)(S^3-3S)=|S|^3-3|S|,
% \]
% we get
% \begin{align*}
%         \E[A_*W]
%         &=\E[(|S|^3-3|S|)\sgn(S^2-r^2)]\\
%         &=2\E[(|S|^3-3|S|)\one_{|S|>r}]
%           -\E[|S|^3-3|S|].
% \end{align*}
% The Gaussian tail moments are
% \[
%         \E[|S|\one_{|S|>r}]=\nu e^{-r^2/2},
%         \qquad
%         \E[|S|^3\one_{|S|>r}]=\nu(r^2+2)e^{-r^2/2}.
% \]
% Also
% \[
%         \E|S|=\nu,
%         \qquad
%         \E|S|^3=2\nu.
% \]
% Therefore
% \begin{align*}
%         \E[A_*W]
%         &=2\nu(r^2-1)e^{-r^2/2}+\nu\\
%         &=\nu\left(1+(1+x)(r^2-1)\right)\\
%         &=\nu\left((1+x)r^2-x\right).
% \end{align*}
% Since $r^2=-2\log((1+x)/2)$,
% \[
%         \E[A_*W]
%         =-\nu\left(x+2(1+x)\log\frac{1+x}{2}\right)
%         =-\nu\Delta(x).
% \]
% This proves the lemma.
% \end{proof}

% \section{Proof of Rearrangement Lemma}
% \label{app:rearrangement_lemma}

% \begin{lemma}[One-dimensional rearrangement]
% Let $S\sim N(0,1)$ and $x\in[0,1]$. Then
% \[
%         \sup_{\substack{|A|\le1\\ \E[A(S)S]=\nu x}}
%         \E[A(S)(S^3-3S)]
%         =-\nu\Delta(x).
% \]
% \end{lemma}

% \begin{proof}
% Fix $r\ge0$ by
% \[
%         e^{-r^2/2}=\frac{1+x}{2},
% \]
% and put
% \[
%         \mu=r^2-3.
% \]
% Let $W=S^3-3S$. Then
% \[
%         W-\mu S=S^3-3S-(r^2-3)S=S(S^2-r^2).
% \]

% For any feasible $A$,
% \begin{align*}
%         \E[AW]
%         &=\E[A(W-\mu S)]+\mu\E[AS]\\
%         &=\E[A(W-\mu S)]+\mu\nu x\\
%         &\le \E|W-\mu S|+\mu\nu x,
% \end{align*}
% using $|A|\le1$.

% Equality is attained by
% \[
%         A_*(S)=\sgn(W-\mu S)=\sgn(S)\sgn(S^2-r^2),
% \]
% provided $A_*$ has the right first moment. It does, because
% \[
%         A_*(S)S=|S|\sgn(S^2-r^2),
% \]
% so
% \begin{align*}
%         \E[A_*(S)S]
%         &=2\E[|S|\one_{|S|>r}]-\E|S|\\
%         &=2\nu e^{-r^2/2}-\nu\\
%         &=\nu x.
% \end{align*}
% Thus $A_*$ is feasible and attains the dual upper bound.

% It remains to compute its value. Since
% \[
%         \sgn(S)(S^3-3S)=|S|^3-3|S|,
% \]
% we get
% \begin{align*}
%         \E[A_*W]
%         &=\E[(|S|^3-3|S|)\sgn(S^2-r^2)]\\
%         &=2\E[(|S|^3-3|S|)\one_{|S|>r}]
%           -\E[|S|^3-3|S|].
% \end{align*}
% The Gaussian tail moments are
% \[
%         \E[|S|\one_{|S|>r}]=\nu e^{-r^2/2},
%         \qquad
%         \E[|S|^3\one_{|S|>r}]=\nu(r^2+2)e^{-r^2/2}.
% \]
% Also
% \[
%         \E|S|=\nu,
%         \qquad
%         \E|S|^3=2\nu.
% \]
% Therefore
% \begin{align*}
%         \E[A_*W]
%         &=2\nu(r^2-1)e^{-r^2/2}+\nu\\
%         &=\nu\left(1+(1+x)(r^2-1)\right)\\
%         &=\nu\left((1+x)r^2-x\right).
% \end{align*}
% Since $r^2=-2\log((1+x)/2)$,
% \[
%         \E[A_*W]
%         =-\nu\left(x+2(1+x)\log\frac{1+x}{2}\right)
%         =-\nu\Delta(x).
% \]
% This proves the lemma.
% \end{proof}


\section{Certification of the Fiber Inequality}
\label{app:fiber-certificate}

This appendix reduces the fiber inequality~\eqref{eq:fiber-inequality},
\[
        V(u)\le 3\nu\beta(u)-\beta(u)^2
        \qquad\text{for every ternary } u:\R\to\{-1,0,1\},
\]
to a finite family of one-dimensional inequalities, and documents the interval-arithmetic certificates that verify each of them. Throughout, $Z\sim N(0,1)$, $\gamma$ is its law, $\varphi(s)=e^{-s^2/2}/\sqrt{2\pi}$, and
\[
        V(u)=\sum_{j=0}^3\E[u\psi_j]^2,
        \qquad
        \beta(u)=\E\bigl[|Z|\,u(Z)^2\bigr]\in[0,\nu].
\]

All computations are performed in Arb ball arithmetic~\cite{johansson2017arb} (via \texttt{python-flint~0.8.0}, the Python interface to FLINT~3, which incorporates Arb; working precision $256$--$400$ bits): every computed quantity is an interval $[\text{mid}\pm\text{rad}]$ whose radius is a rigorous outward-rounded error bound, and an inequality counts as \emph{certified} only when the entire interval lies on the claimed side of $0$. All certificates are deterministic. The scripts, their logs, and a one-command driver are collected in the repository directory \texttt{lower\_bound\_reproducibility/}; script names below refer to its \texttt{scripts/} folder.

\subsection{Reduction to two certified regimes}
\label{app:fq1-reduction}

The budget axis $\beta\in[0,\nu]$ is covered by two regimes: a direction-free bound for large budgets, and a Fenchel-dual bound for small budgets. Write
\[
        \phi(\beta):=\sqrt{3\nu\beta-\beta^2},
\]
so that~\eqref{eq:fiber-inequality} is exactly $\sqrt{V(u)}\le\phi(\beta(u))$.

\begin{lemma}[High-budget regime]\label{lem:highbudget}
Let $u$ be ternary with $\beta(u)=\beta\in(0,\nu]$, and let $r\in(0,\infty]$ solve $\nu(1-e^{-r^2/2})=\beta$. Then
\[
        V(u)\;\le\;\Pr(u\neq0)\;\le\;2\PhiG(r)-1 .
\]
Consequently, if
\begin{equation}
        g(r):=3\nu\beta(r)-\beta(r)^2-\bigl(2\PhiG(r)-1\bigr)\;\ge\;0,
        \qquad \beta(r):=\nu(1-e^{-r^2/2}),
        \label{eq:g-def}
\end{equation}
then~\eqref{eq:fiber-inequality} holds for $u$.
\end{lemma}

\begin{proof}
The first inequality is Bessel: $\psi_0,\ldots,\psi_3$ are orthonormal, so $V(u)\le\norm{u}_2^2=\E[u^2]=\Pr(u\neq0)$. The second is the bathtub principle already used in Section~\ref{sec:disagreement}: among all supports $E$ with $\int_E|s|\,d\gamma=\beta$, the Gaussian measure $\gamma(E)$ is maximized by the centered interval $E_r=\{|s|\le r\}$ with the same budget. Indeed $(\one_E-\one_{E_r})(|s|-r)\ge0$ pointwise, and integrating gives $0\le 0-r(\gamma(E)-\gamma(E_r))$, i.e.\ $\gamma(E)\le\gamma(E_r)=2\PhiG(r)-1$.
\end{proof}

\begin{lemma}[Dual regime and the Fenchel splice]\label{lem:dual-splice}
Call $p=\sum_{j=0}^3a_j\psi_j$ with $\norm{a}_2=1$ a \emph{unit cubic}, and set
\[
        J(c,p):=\E\bigl[(|p(Z)|-c|Z|)_+\bigr],
        \qquad
        d(c):=\frac{3\nu}{2}\bigl(\sqrt{1+c^2}-c\bigr),
        \qquad
        \beta_*(c):=\frac{3\nu}{2}\Bigl(1-\frac{c}{\sqrt{1+c^2}}\Bigr).
\]
Fix $c_M>0$ and suppose that
\begin{equation}
        J(c,p)\le d(c)
        \qquad\text{for every unit cubic } p \text{ and every } c\ge c_M.
        \label{eq:dual-bound}
\end{equation}
Then~\eqref{eq:fiber-inequality} holds for every ternary $u$ with $\beta(u)\le\beta_*(c_M)$.
\end{lemma}

\begin{proof}
Let $v_j=\E[u\psi_j]$ and $m=\norm{v}_2=\sqrt{V(u)}$. If $m=0$ there is nothing to prove, since $3\nu\beta-\beta^2=\beta(3\nu-\beta)\ge0$ on $[0,\nu]$. Otherwise $p=\sum_j(v_j/m)\psi_j$ is a unit cubic with $m=\E[u\,p]$, and for every $c\ge0$,
\[
        m=\E[u\,p]\le\int_{\{u\neq0\}}|p|\,d\gamma
        \le\int(|p|-c|s|)_+\,d\gamma+c\int_{\{u\neq0\}}|s|\,d\gamma
        =J(c,p)+c\,\beta(u).
\]
Next, $d$ is the concave conjugate of $\phi$: since $\phi(\beta)^2+(\beta-\tfrac{3\nu}{2})^2=(\tfrac{3\nu}{2})^2$, the graph of $\phi$ is the upper semicircle of radius $R=\tfrac{3\nu}{2}$ centered at $(R,0)$, whence
\[
        \sup_{0\le\beta\le2R}\bigl(\phi(\beta)-c\beta\bigr)=R\bigl(\sqrt{1+c^2}-c\bigr)=d(c),
\]
attained at the tangency budget $\beta=\beta_*(c)$. The map $c\mapsto\beta_*(c)$ is a strictly decreasing bijection from $[0,\infty)$ onto $(0,R]$, so for $\beta\le\beta_*(c_M)$ the tangent slope $c(\beta)=\beta_*^{-1}(\beta)$ satisfies $c(\beta)\ge c_M$, and biconjugation on the semicircle gives
\[
        \inf_{c\ge c_M}\bigl(d(c)+c\beta\bigr)=d\bigl(c(\beta)\bigr)+c(\beta)\,\beta=\phi(\beta).
\]
Combining, $m\le\phi(\beta(u))$, i.e.\ $V(u)=m^2\le3\nu\beta(u)-\beta(u)^2$. (For $\beta(u)=0$ the same chain gives $m\le\inf_{c\ge c_M}d(c)=0$, using~\eqref{eq:dual-bound} for arbitrarily large $c$.)
\end{proof}

\begin{remark}[Exactness of the threshold reduction]\label{rem:exactness}
The step $m\le J(c,p)+c\beta(u)$ is the easy half of an exact pointwise duality: for every $z$,
\[
        \max_{v\in\{-1,0,1\}}\bigl(v\,p(z)-c|z|\,v^2\bigr)=\bigl(|p(z)|-c|z|\bigr)_+,
\]
with maximizer $v(z)=\sgn(p(z))\one_{\{|p(z)|\ge c|z|\}}$, so that in fact
\[
        \sup_{u\ \text{ternary}}\bigl(\E[u\,p]-c\,\beta(u)\bigr)=J(c,p),
\]
attained by the threshold rule. The dual gate~\eqref{eq:dual-bound} is therefore not a lossy relaxation of the small-budget regime: it says precisely that every priced threshold optimum lies below the corresponding tangent line of the semicircle.
\end{remark}

\begin{proposition}[Coverage]\label{prop:fq1-coverage}
Take $c_M=0.993405$. The certificates of Sections~\ref{app:cert-highbeta}--\ref{app:cert-highc} establish:
\begin{enumerate}
\item[\textup{(C1)}] $g\ge0$ on $[r_1,\infty]$ with $r_1=1.081596$; hence, by Lemma~\ref{lem:highbudget}, \eqref{eq:fiber-inequality} holds whenever $\beta(u)\ge\beta_0:=\beta(r_1)$, with the certified enclosure $\beta_0=0.353345035094\pm4.4\times10^{-13}$;
\item[\textup{(C2)}, \textup{(C3)}] the dual bound~\eqref{eq:dual-bound} for all $c\in[c_M,12]$ and all $c\ge12$ respectively;
\item[\textup{(S)}] the splice inequality $\beta_0\le\beta_*(c_M)$, with certified enclosures $\beta_*(c_M)=0.353346937306\pm1.1\times10^{-13}$ and $\beta_*(c_M)-\beta_0=1.9022\times10^{-6}\pm3.9\times10^{-14}>0$.
\end{enumerate}
Since $[0,\beta_*(c_M)]\cup[\beta_0,\nu]=[0,\nu]$, the fiber inequality~\eqref{eq:fiber-inequality} holds for every ternary $u$.
\end{proposition}

Everything that remains is finite: (C1) is a one-variable inequality on a half-line, (S) is a single sign check, and (C2)--(C3) are inequalities over compact parameter sets --- the medium regime is certified on $S^3\times[c_M,12]$, and in the tail regime the change of variables $\lambda=1/c$ turns $c\ge12$ into the compact range $S^3\times[0,\tfrac1{12}]$, with the endpoint $\lambda=0$ handled through the scaled Taylor expansion of Section~\ref{app:cert-highc}. The next three subsections describe exactly what is checked in each case.

\subsection{Certificate (C1): the high-budget inequality}
\label{app:cert-highbeta}

Differentiating~\eqref{eq:g-def} and using $2\varphi(r)=\nu e^{-r^2/2}$,
\[
        g'(r)=2\varphi(r)\,B(r),
        \qquad
        B(r)=r\nu\bigl(1+2e^{-r^2/2}\bigr)-1,
        \qquad
        B'(r)=\nu\Bigl(1-2e^{-r^2/2}(r^2-1)\Bigr).
\]
The function $2e^{-r^2/2}(r^2-1)$ is maximized at $r^2=3$, where it equals $4e^{-3/2}$; the certified check $4e^{-3/2}<1$ therefore gives $B'>0$ for all $r\ge1$. Consequently the two thin-ball checks
\[
        g(r_1)>0,\qquad B(r_1)>0 \qquad (r_1=1.081596)
\]
prove $g'\ge0$ hence $g\ge g(r_1)>0$ on all of $[r_1,\infty)$, and the certified limit $g(\infty)=2\nu^2-1>0$ covers $\beta=\nu$. The script \texttt{highbeta\_monotone.py} (prec.\ $300$) certifies all four facts, obtaining
\[
        g(r_1)=3.65\times10^{-4}\pm2.1\times10^{-7},
        \qquad
        B(r_1)=0.824613\pm3.7\times10^{-7},
        \qquad
        4e^{-3/2}=0.89252\ldots<1,
\]
together with an independent (logically redundant) interval scan certifying $B'>0$ on $[1,8)$. A second script, \texttt{highbeta\_refine.py} (prec.\ $400$), supplies the splice constants: it computes the certified enclosures of $\beta_0=\beta(r_1)$ and $\beta_*(c_M)$ quoted in Proposition~\ref{prop:fq1-coverage} and certifies the splice inequality (S), re-verifying $g\ge0$ on $[r_1,\,1.0816]$ with fine interval balls along the way.

\subsection{Certificate (C2): the dual envelope on the medium band $c\in[c_M,12]$}
\label{app:cert-envelope}

Fold $J$ onto the half-line and split $p=e+o$ into its even part $e=a_0\psi_0+a_2\psi_2$ and odd part $o=a_1\psi_1+a_3\psi_3$:
\begin{equation}
        J(c,p)=\int_0^\infty\Bigl[\bigl(|p(s)|-cs\bigr)_++\bigl(|p(-s)|-cs\bigr)_+\Bigr]\varphi(s)\,ds ,
        \label{eq:J-fold}
\end{equation}
and for each $s$ the unordered pair $\{|p(s)|,|p(-s)|\}$ equals $\{|e(s)|+|o(s)|,\;\bigl||e(s)|-|o(s)|\bigr|\}$ (because $|e\pm o|$ take exactly these two values in some order). The integrand of~\eqref{eq:J-fold} is therefore $f\bigl(|e(s)|,|o(s)|\bigr)$ with
\[
        f(x,y):=(x+y-t)_++\bigl(|x-y|-t\bigr)_+,\qquad t=cs\ge0 .
\]

\begin{lemma}[Envelope monotonicity]\label{lem:fold-mono}
For every $t\ge0$, the function $f$ is nondecreasing in each of $x\ge0$ and $y\ge0$. Hence $f\bigl(|e(s)|,|o(s)|\bigr)\le f\bigl(\bar A(s),\omega(s)\bigr)$ for any pointwise upper bounds $\bar A\ge|e|$, $\omega\ge|o|$.
\end{lemma}

\begin{proof}
$f$ is symmetric in $(x,y)$, so it suffices to treat $x$; fix $y$ and distinguish the three regimes of the second term. If $x-y>t$, both terms are active (as $x+y\ge x-y>t$) and the $x$-slope is $1+1=2$. If $y-x>t$, both terms are again active ($x+y>2x+t\ge t$) and the slopes cancel, $1-1=0$. If $|x-y|\le t$, the second term vanishes and $f=(x+y-t)_+$ has $x$-slope $0$ or $1$. In every case the slope is $\ge0$.
\end{proof}

The certificate applies Lemma~\ref{lem:fold-mono} with the Cauchy--Schwarz (Christoffel) envelopes

\begin{align*}
        |o(s)|&\le r_o\sqrt{K_o(s)},
        & K_o&=\psi_1^2+\psi_3^2=\tfrac{5}{2}s^2-s^4+\tfrac16 s^6,\\
        |e(s)|&\le|e_{\bar a}(s)|+\rho\sqrt{K_e(s)},
        & K_e&=\psi_0^2+\psi_2^2=\tfrac32-s^2+\tfrac12 s^4,
\end{align*}
where $\bar a=(\bar a_0,\bar a_2)$ is the center of an even-coefficient box of circumradius $\rho$, and $r_o=\sqrt{1-l^2}$ with $l=\max(0,\norm{\bar a}-\rho)$ bounds the odd-coefficient norm of \emph{any} unit cubic whose even part lies in the box. In this way a single evaluation certifies the box against \emph{all} compatible odd parts, and the search space is the two-dimensional even disk rather than $S^3$ (by $J(c,-p)=J(c,p)$ one may take $a_0\ge0$).

The integral~\eqref{eq:J-fold} is enclosed by $480$ interval panels on $s\in[0,8]$ (per-panel ball enclosures of $f(\bar A,\omega)$ times upper bounds of the panel's Gaussian weight, all roundings outward) plus the closed-form tail majorant
\[
        \int_8^\infty\Bigl(1+\tfrac{s^2+1}{\sqrt2}+s^3\Bigr)\varphi(s)\,ds\;\le\;3.7\times10^{-13}
        \qquad(\text{the integral is }\approx3.64\times10^{-13}).
\]
The majorant is valid because $f(x,y)\le(x+y)+|x-y|=2\max\{x,y\}$, while for $s\ge8$ both $|e|\le1+(s^2+1)/\sqrt2\le s^3/2$ and $|o|\le\sqrt{K_o}\le s^3/\sqrt6\le s^3/2$, so the folded integrand is at most $s^3\le1+\tfrac{s^2+1}{\sqrt2}+s^3$; the scripts use the rigorous Arb enclosure of the tail integral, not the rounded decimal above. On a $c$-band $[c_L,c_U]$ the certificate uses the monotonicities $J(c,p)\le J(c_L,p)$ and $d(c)\ge d(c_U)$, so certifying $\overline{U}(\text{box},c_L)\le\underline{d}(c_U)$ certifies all $c$ in the band at once. The branch-and-bound starts from a grid of spacing $0.08$ on the even disk whose boxes have half-width equal to the spacing (so they cover the disk with twofold overlap), splits any uncertified box into four (down to a failure floor of half-width $6\times10^{-4}$, never reached), and subdivides $c$-bands geometrically on failure.

Run as eight parallel sub-bands whose union is $[c_M,12]$ with no hole (bands~6 and~7 overlap on $[4.0,4.083]$), the certificate resolves $95{,}784$ boxes in about $30$ seconds and certifies~\eqref{eq:dual-bound} on the whole band; per-band results are listed in Table~\ref{tab:fq1-bands}. The worst certified margin over the tiling, $+2.26\times10^{-5}$, measures the tightness of the \emph{envelope relaxation}, not of~\eqref{eq:fiber-inequality} (see the remark at the end of this appendix); it grows under finer $c$-banding.

\begin{table}[h]\centering
\begin{tabular}{lllll}
\hline
band & $c$-range & sub-bands & boxes & worst certified margin \\
\hline
1 & $[0.993405,\,1.19]$ & 12 & 12{,}164 & $+1.088\times10^{-4}$ \\
2 & $[1.19,\,1.30]$ & 14 & 12{,}416 & $+9.058\times10^{-5}$ \\
3 & $[1.30,\,1.45]$ & 12 & 10{,}712 & $+8.958\times10^{-5}$ \\
4 & $[1.45,\,1.75]$ & 8 & 7{,}988 & $+1.956\times10^{-4}$ \\
5 & $[1.75,\,3.5]$ & 24 & 24{,}200 & $+2.260\times10^{-5}$ \\
6 & $[3.5,\,4.083]$ & 10 & 7{,}584 & $+2.830\times10^{-5}$ \\
7 & $[4.0,\,6.0]$ & 16 & 11{,}840 & $+3.571\times10^{-5}$ \\
8 & $[6.0,\,12.0]$ & 14 & 8{,}880 & $+2.539\times10^{-5}$ \\
\hline
\end{tabular}
\caption{Certificate (C2): the eight sub-bands of the dual-envelope branch-and-bound (\texttt{envelope\_band.py}, precision $256$ bits). Each row certifies $J(c,p)\le d(c)$ for \emph{all} unit cubics $p$ and all $c$ in its range; ``sub-bands'' is the geometric $c$-tiling within the row.}
\label{tab:fq1-bands}
\end{table}

\subsection{Certificate (C3): the high-$c$ tail $c\ge12$}
\label{app:cert-highc}

For $c\ge12$ substitute $\lambda=1/c\in(0,\tfrac1{12}]$ and $x=cs$. Both sides of~\eqref{eq:dual-bound} then carry a factor $\lambda$: after dividing it out, the target becomes $D(\lambda)\ge I(\lambda,p)$ with
\[
        D(\lambda)=\frac{3\nu}{2}\cdot\frac{1}{1+\sqrt{1+\lambda^2}},
        \qquad
        I(\lambda,p)=\int_0^\infty\Bigl[\bigl(|p(\lambda x)|-x\bigr)_++\bigl(|p(-\lambda x)|-x\bigr)_+\Bigr]\varphi(\lambda x)\,dx .
\]
As $\lambda\downarrow0$ this degenerates, and it is worth seeing why. For large $c$ the active condition $|p(s)|\ge c|s|$ selects a small neighbourhood of the origin, where $J(c,p)=\varphi(0)\,p(0)^2/c+O(c^{-3})$. Among unit cubics the largest possible value of $p(0)^2$ is the evaluation-kernel norm $K_{\le3}(0,0)=\sum_{j\le3}\psi_j(0)^2=\tfrac32$, attained by the normalized reproducing kernel at the origin,
\[
        p_0(s)=\frac{K_{\le3}(s,0)}{\sqrt{K_{\le3}(0,0)}}=\frac{3-s^2}{\sqrt6}=\sqrt{\tfrac23}\,\psi_0-\tfrac{1}{\sqrt3}\,\psi_2 .
\]
Since $\varphi(0)=\nu/2$, this gives $\sup_pJ(c,p)\sim\tfrac{3\nu}{4c}$, while also $d(c)\sim\tfrac{3\nu}{4c}$: \emph{the dual bound is asymptotically tight}, with equality direction $p_0$. In the scaled variables, $D(0)=I(0,p_0)=\tfrac34\nu$, and the margin vanishes to second order in $\lambda$. This is why the tail cannot be closed by more branch-and-bound---near the limit every box fails---and why the certified object is instead the scaled margin $\bigl(D-I\bigr)/\lambda^2$, which has a strictly positive limit. For orientation (this computation is cross-checked numerically but not used below): in the local chart introduced next,
\[
        \frac{D(\lambda)-I(\lambda,p)}{\lambda^2}
        \;\longrightarrow\;
        \frac{5\nu}{32}+\frac{3\nu}{4}\norm{y}^2
        \qquad(\lambda\downarrow0),
\]
and the certified leading jets of the majorant constructed below reproduce exactly these values minus the far-tail reserve of Lemma~\ref{lem:remote-tail} ($0.094669=\tfrac{5\nu}{32}-0.03$ at $y=0$; increment $0.598414=\tfrac{3\nu}{4}$ at $y=(0,0,1)$), confirming that the majorant is lossless at leading order.

Every unit cubic with $q:=|\ip{p}{p_0}|>0$ can be written (up to sign) in the \emph{local chart}
\[
        p=\frac{p_0+\lambda\,w}{\sqrt{1+\lambda^2\norm{y}^2}},
        \qquad
        w=y_E\,\frac{s^2}{\sqrt3}+y_1\psi_1+y_3\psi_3\perp p_0,
        \qquad
        \norm{w}=\norm{y},
\]
and the transverse coordinate $z:=(1-q^2)/\lambda^2$ satisfies $z=\norm{y}^2/(1+\lambda^2\norm{y}^2)$. The certificate covers all $p$ by two overlapping charts:
\begin{itemize}
\item \textbf{LOCAL} ($\norm{y}\le2$, equivalently $z\le4/(1+4\lambda^2)\ge3.891$ for $\lambda\le\tfrac1{12}$);
\item \textbf{AWAY} ($z\in[3.88,4.2]$ by branch-and-bound in $z$, and $z\ge4.2$ by a certified monotone-domination bracket); this includes $q=0$, where $z=c^2\ge144$.
\end{itemize}
Since $3.88<3.891$ the union covers every $z\ge0$, i.e.\ every unit cubic, for every $c\ge12$.

\subsubsection*{Localization and the far tail}

The active sets $\{x:|p(\pm\lambda x)|\ge x\}$ are \emph{not} compact in the scaled variable: a genuine cubic grows like $\lambda^3x^3$, so the active condition, which for moderate $x$ holds only in a central window, holds again on a remote ray (for $p=\psi_3$ and $\lambda=\tfrac1{12}$ the re-entry is near $x\approx68$). The certificate separates the two components and covers the remote one by an explicit allowance.

\begin{lemma}[Localization]\label{lem:localization}
Let $K(s):=\sum_{j=0}^3\psi_j(s)^2=\tfrac32+\tfrac32s^2-\tfrac12s^4+\tfrac16s^6$. For every unit cubic $p$, every $c\ge12$ and every $s\ge0$: if $|p(s)|\ge cs$, then
\[
        cs<1.5\;(<L:=1.55)
        \qquad\text{or}\qquad
        s>1.55\sqrt c .
\]
\end{lemma}

\begin{proof}
Cauchy--Schwarz gives $|p(s)|^2\le K(s)$, so activity implies $F_c(s^2)\le0$, where $F_c(x):=c^2x-\bigl(\tfrac32+\tfrac32x-\tfrac12x^2+\tfrac16x^3\bigr)$. It therefore suffices that $F_c>0$ on $[(1.5/c)^2,\,1.55^2c]$. Since $F_c'(x)=c^2-\tfrac32+x-\tfrac{x^2}2$ is a downward parabola in $x$, positive at the left endpoint, $F_c$ is increasing-then-decreasing on the interval, so its minimum is attained at an endpoint. At the left endpoint, $F_c\bigl((1.5/c)^2\bigr)=\tfrac34-\tfrac32u+\tfrac{u^2}2-\tfrac{u^3}6$ with $u=2.25/c^2\in(0,\tfrac1{64}]$, certified positive over the whole $u$-range; at the right endpoint, $G(c):=F_c(1.55^2c)$ is a cubic in $c$ with positive leading coefficient $1.55^2(1-1.55^4/6)$ and certified $G(12)>0$, $G'(12)>0$ (and $G'$ is increasing), so $G>0$ for all $c\ge12$. The three sign evaluations are certified in \texttt{highc\_remote\_tail.py}.
\end{proof}

\begin{lemma}[Far-tail allowance]\label{lem:remote-tail}
For every unit cubic $p$ and every $c\ge12$,
\[
        J_{\mathrm{rem}}(c,p):=\int_{\{|s|\ge1.55\sqrt c\}}\bigl(|p(s)|-c|s|\bigr)_+\,d\gamma
        \;\le\;2\bigl(1.55^2c+2\bigr)\,\varphi\bigl(1.55\sqrt c\bigr)
        \;\le\;\frac{0.03}{c^3};
\]
equivalently, the remote active components contribute at most $0.03\lambda^2$ to $I(\lambda,p)$.
\end{lemma}

\begin{proof}
For $s\ge2$ one has $K(s)\le s^6$ (equivalent to $9+9s^2\le3s^4+5s^6$, true since $3s^4\ge12s^2>9s^2+9$), so on the remote set $\bigl(|p(s)|-c|s|\bigr)_+\le\sqrt{K(s)}\le s^3$; applying $\int_a^\infty s^3\varphi\,ds=(a^2+2)\varphi(a)$ on both half-lines gives the first bound. For the second, set $t(c):=c^3\cdot2(1.55^2c+2)\varphi(1.55\sqrt c)$; then
\[
        (\ln t)'(c)=\frac3c+\frac{1.55^2}{1.55^2c+2}-\frac{1.55^2}2
        \;\le\;\frac3{12}+\frac{1.55^2}{12\cdot1.55^2+2}-\frac{1.55^2}2\;<\;-0.87,
\]
so $t$ is decreasing on $[12,\infty)$; the certified value $t(12)=0.0233\ldots<0.03$ completes the proof. Both sign checks are certified in \texttt{highc\_remote\_tail.py}.
\end{proof}

This is the exact role of the reserve $0.03\lambda^2$ deducted inside the certified functionals below: it pays for the far tail, so that certifying the central majorant against $D-0.03\lambda^2$ certifies all of~\eqref{eq:dual-bound}. The central window is then frozen at the fixed cutoff $A:=p_0(0)=\sqrt{3/2}$ (the limiting active boundary, since $p_0(0)=x$ at $x=A$) by the following device, which avoids an interval-unstable moving root:

\begin{lemma}[Moving cutoff]\label{lem:moving-cutoff}
Let $0\le w(x)\le\varphi_0:=1/\sqrt{2\pi}$, let $\delta:[0,L]\to\R$ be measurable with $|\delta|\le\Delta$, and let $0<A\le L$. Then
\[
        \int_0^L\bigl(A-x+\delta(x)\bigr)_+\,w(x)\,dx
        \;\le\;
        \int_0^A\bigl(A-x+\delta(x)\bigr)\,w(x)\,dx+\varphi_0\Delta^2 .
\]
\end{lemma}

\begin{proof}
On $[0,A]$, $(A-x+\delta)_+-(A-x+\delta)=(x-A-\delta)_+\le(x-A+\Delta)_+$, which is supported on $[A-\Delta,A]$ and bounded by $\Delta$; its $w$-integral is at most $\varphi_0\Delta^2/2$. On $[A,L]$, $(A-x+\delta)_+\le(\Delta-(x-A))_+$, again contributing at most $\varphi_0\Delta^2/2$.
\end{proof}

\subsubsection*{The LOCAL majorant}

In the local chart, with $n:=\sqrt{1+\lambda^2\norm{y}^2}$,
\[
        n\,p(\pm\lambda x)=P_\pm(x)
        :=A-\frac{\lambda^2x^2}{\sqrt6}+\frac{y_E\lambda^3x^2}{\sqrt3}
        \pm\lambda^2\Bigl(y_1x+y_3\,\frac{\lambda^2x^3-3x}{\sqrt6}\Bigr).
\]
An interval evaluation certifies $P_\pm/n>0$ for $x\in[0,L]$, $\lambda\in[0,\tfrac1{12}]$ and the whole $y$-range, so there $|p(\pm\lambda x)|=P_\pm(x)/n$; by Lemmas~\ref{lem:localization} and~\ref{lem:remote-tail},
\begin{equation}
        I(\lambda,p)\;\le\;\int_0^L\Bigl[\Bigl(\frac{P_+}{n}-x\Bigr)_++\Bigl(\frac{P_-}{n}-x\Bigr)_+\Bigr]\varphi(\lambda x)\,dx
        \;+\;0.03\lambda^2 .
        \label{eq:reserve}
\end{equation}
Write $P_\pm/n-x=A-x+\delta_\pm(x)$ with $\delta_\pm:=P_\pm/n-A$, and apply Lemma~\ref{lem:moving-cutoff} to each branch with weight $w=\varphi(\lambda\,\cdot)\le\varphi_0$. In $\sum_\pm\int_0^A\delta_\pm w$ the $y_1,y_3$ terms cancel (they are odd under the branch sign), leaving, with the frozen moments $W_j(\lambda):=\int_0^Ax^j\varphi(\lambda x)\,dx$,
\[
        \int_0^L\Bigl[\,\cdots\Bigr]\varphi(\lambda x)\,dx
        \;\le\;U_{\mathrm{loc}}
        :=2\bigl(AW_0-W_1\bigr)+2A\Bigl(\frac1n-1\Bigr)W_0
        -\frac{2\lambda^2}{\sqrt6\,n}W_2+\frac{2y_E\lambda^3}{\sqrt3\,n}W_2
        +\varphi_0\bigl(\Delta_+^2+\Delta_-^2\bigr),
\]
where $\Delta_\pm\ge\sup_{[0,L]}|\delta_\pm|$ is supplied by the split $\Delta_\pm=M_E+M_O$ into branch-even and branch-odd parts,
\[
        M_E=A\Bigl(1-\frac1n\Bigr)+\frac{\lambda^2L^2}{\sqrt6\,n}+\frac{|y_E|\,\lambda^3L^2}{\sqrt3\,n},
        \qquad
        M_O=\frac{\lambda^2\norm{y}L}{n}\sqrt{\tfrac52}\,.
\]
$M_E$ bounds the branch-even part of $\delta_\pm$ termwise on $[0,L]$; $M_O$ bounds the branch-odd part by Cauchy--Schwarz,
\[
        \Bigl|y_1x+y_3\,\frac{\lambda^2x^3-3x}{\sqrt6}\Bigr|
        =\frac{\bigl|y_1\psi_1(\lambda x)+y_3\psi_3(\lambda x)\bigr|}{\lambda}
        \le\frac{\norm{y}}{\lambda}\sqrt{K_o(\lambda x)}
        \le x\norm{y}\sqrt{\tfrac52},
\]
using $K_o(s)=s^2\bigl(1+\tfrac{(3-s^2)^2}{6}\bigr)\le\tfrac52s^2$ for $s^2\le6$; an interval check certifies $s^2=\lambda^2x^2\le0.017$ on the chart, so the condition holds with a wide margin.

\subsubsection*{The AWAY majorant}

Here only the size of the transverse part enters, not its direction. Write $p=\pm(q\,p_0+\tau)$ with $\tau\perp p_0$, $q=\sqrt{1-\lambda^2z}$ and $\norm{\tau}=\lambda\sqrt z$, and let
\[
        K_\perp(s):=K(s)-p_0(s)^2=\tfrac52s^2-\tfrac23s^4+\tfrac16s^6\;\le\;\tfrac52s^2
        \qquad(s^2\le4).
\]
Then $|\tau(\pm\lambda x)|\le\lambda\sqrt z\,\sqrt{K_\perp(\lambda x)}\le\lambda^2x\sqrt{5z/2}$, so both branches obey the same bound $|p(\pm\lambda x)|-x\le A-x+\delta_z(x)$ with
\[
        \delta_z(x)=A(q-1)-\frac{q\lambda^2x^2}{\sqrt6}+\lambda^2x\sqrt{\tfrac{5z}2}
\]
(no branch-positivity check is needed here, because $|p|$ is bounded from above directly). Lemma~\ref{lem:moving-cutoff} applied to both branches then gives
\[
        U_{\mathrm{away}}
        =2\bigl(AW_0-W_1\bigr)+2\Bigl(A(q-1)W_0-\frac{q\lambda^2}{\sqrt6}W_2+\lambda^2\sqrt{\tfrac{5z}2}\,W_1\Bigr)
        +2\varphi_0M_z^2,
\]
with $M_z=A(1-q)+\dfrac{\lambda^2L^2}{\sqrt6}+\lambda^2L\sqrt{\dfrac{5z}2}\;\ge\;\sup_{[0,L]}|\delta_z|$ (using $q\le1$). Finally, $z\ge4.2$ is reduced to the certified band by domination:

\begin{lemma}[Domination for $z\ge z_0=4.2$]\label{lem:domination}
Let $a_z(x):=\sqrt{1-\lambda^2z}\,p_0(\lambda x)+\lambda\sqrt z\,\sqrt{K_\perp(\lambda x)}$ denote the amplitude bound above, and let
\[
        \widetilde K_\perp(\lambda,x):=\frac{K_\perp(\lambda x)}{\lambda^2}
        =\tfrac52x^2-\tfrac23\lambda^2x^4+\tfrac16\lambda^4x^6,
\]
a polynomial in $(\lambda,x)$ (the continuous extension to $\lambda=0$). If
\[
        z_0\,p_0(\lambda x)^2\;\ge\;\widetilde K_\perp(\lambda,x)\,\bigl(1-z_0\lambda^2\bigr)
        \qquad\text{for all }\lambda\in[0,\tfrac1{12}],\ x\in[0,L],
\]
then $\partial_za_z(x)\le0$ for every $z\ge z_0$ and $\lambda\in(0,\tfrac1{12}]$; hence every $z\ge z_0$ (including $q=0$, i.e.\ $z=c^2$) is pointwise dominated by $z=z_0$, which lies inside the certified band $[3.88,4.2]$.
\end{lemma}

\begin{proof}
For $\lambda>0$, $\partial_za_z=-\dfrac{\lambda^2p_0}{2\sqrt{1-\lambda^2z}}+\dfrac{\lambda\sqrt{K_\perp}}{2\sqrt z}\le0$ iff $\lambda^2z\,p_0^2\ge(1-\lambda^2z)K_\perp(\lambda x)$, i.e.\ (dividing by $\lambda^2$) iff $z\,p_0^2\ge\widetilde K_\perp\,(1-z\lambda^2)$. The displayed hypothesis is this condition at $z=z_0$; as $z$ grows the left side increases and the right side decreases, so it persists for all $z\ge z_0$. The hypothesis is certified on an interval grid with worst lower bound $+0.29$ (\texttt{highc\_certificate.py}).
\end{proof}

\subsubsection*{Evaluation and results}

Each frozen moment is an entire function of $\lambda^2$,
\[
        W_j(\lambda)=\varphi_0\sum_{m\ge0}\frac{(-1)^m}{2^m\,m!}\,\frac{A^{\,j+2m+1}}{j+2m+1}\,\lambda^{2m},
\]
evaluated through the terms $m\le9$, and the omitted tail must be accounted for \emph{with its power of $\lambda$}. It is an alternating series with decreasing terms (successive ratios are at most $\lambda^2A^2/2\le\tfrac1{192}$), hence dominated by its first term:
\[
        \bigl|W_j(\lambda)-\widehat W_j(\lambda)\bigr|
        \;\le\;\varphi_0\,\frac{(A^2/2)^{10}}{10!}\,\frac{A^{\,j+1}}{j+21}\,\lambda^{20}
        \;\le\;10^{-9}\,\lambda^{20}
        \qquad(0\le j\le3),
\]
where $\widehat W_j$ denotes the truncation. The $W_j$ enter $U_{\mathrm{loc}}$ and $U_{\mathrm{away}}$ affinely, with coefficient magnitudes summing to less than $10$, so the truncation perturbs $G$ by at most $10^{-8}\lambda^{20}$ and the scaled margin $R=G/\lambda^2$ by at most $10^{-8}\lambda^{18}\le10^{-27}$, \emph{uniformly} on $(0,\tfrac1{12}]$: the $\lambda^{20}$ factor survives the division by $\lambda^2$, so the comparison is scale-aware and negligible against the certified margins below (all $\ge4\times10^{-3}$). With these ingredients, $G:=D-U_{\mathrm{loc/away}}-0.03\lambda^2$ is an explicit algebraic expression in $\lambda$, and a rigorous lower bound for $R:=G/\lambda^2$, \emph{uniform in} $\lambda\in(0,\tfrac1{12}]$, is obtained from the Taylor jet of $G$ at $\lambda=0$ (Arb series coefficients) plus a Lagrange remainder enclosed by the corresponding ball-centered jet over $[0,\tfrac1{12}]$, for each interval box of chart parameters. By~\eqref{eq:reserve} and its AWAY analogue, certifying $R>0$ certifies $D-I>0$, i.e.~\eqref{eq:dual-bound}, on the box.

The branch-and-bound (\texttt{highc\_certificate.py}, precision $300$ bits) certifies: LOCAL, $R>0$ over the ball $\norm{y}\le2$ ($1{,}000$ certified boxes, $1{,}319$ subdivisions, $\approx1$ s), worst certified value $+4.211\times10^{-3}$; AWAY, $R>0$ on $z\in[3.88,4.2]$ (certified in a single interval evaluation), worst $+3.537\times10^{-2}$, together with the domination bracket of Lemma~\ref{lem:domination} and the range check for $M_O$; and the localization and far-tail constants of Lemmas~\ref{lem:localization}--\ref{lem:remote-tail} are certified in \texttt{highc\_remote\_tail.py}.

\subsection{Summary of certified results and reproducibility}
\label{app:cert-summary}

\begin{table}[h]\centering
\footnotesize
\setlength{\tabcolsep}{4pt}
\begin{tabular}{llll}
\hline
certificate & script(s) & what is certified & worst margin \\
\hline
(C1) point $+$ monot. & \texttt{highbeta\_monotone.py} & $g(r_1)>0$, $B(r_1)>0$, $4e^{-3/2}<1$, $g(\infty)>0$ & $+3.65\times10^{-4}$ \\
(C1)$+$(S) fine scan & \texttt{highbeta\_refine.py} & $g\ge0$ on $[r_1,1.0816]$; $\beta_0<\beta_*(c_M)$ & $+1.90\times10^{-6}$ \\
(C2) medium band & \texttt{envelope\_band.py} $\times8$ & $J(c,p)\le d(c)$, all $p\in S^3$, $c\in[c_M,12]$ & $+2.26\times10^{-5}$ \\
(C3) tail, LOCAL & \texttt{highc\_certificate.py} & $R>0$, $\norm{y}\le2$, $\lambda\in(0,\tfrac1{12}]$ & $+4.21\times10^{-3}$ \\
(C3) tail, AWAY & \texttt{highc\_certificate.py} & $R>0$, $z\in[3.88,4.2]$; domination $z\ge4.2$ & $+3.54\times10^{-2}$ \\
(C3) far tail & \texttt{highc\_remote\_tail.py} & active: $cs<1.5$ or $s>1.55\sqrt c$; $J_{\mathrm{rem}}\le0.03c^{-3}$ & $+6.66\times10^{-3}$ \\
\hline
\end{tabular}
\caption{The fiber-inequality certificate, region by region (run of 2026-08-04; all margins are rigorous one-sided ball bounds). Together with Lemmas~\ref{lem:highbudget} and~\ref{lem:dual-splice} these establish~\eqref{eq:fiber-inequality} for every ternary $u$ via Proposition~\ref{prop:fq1-coverage}.}
\label{tab:fq1-results}
\end{table}

Table~\ref{tab:fq1-results} summarizes the certificate. The complete suite runs in under two minutes on one machine via the driver \texttt{run\_all.sh} of \texttt{lower\_bound\_reproducibility/}, which executes every script, stores the logs under \texttt{certificates/}, and verifies the certified verdict line of each log; the only requirement is Python~$\ge3.11$ with \texttt{python-flint~0.8.0}. Every certificate is deterministic: re-runs in the pinned environment reproduce the printed margins verbatim, and independent environments must reproduce the same certified verdicts and enclosures.

\begin{remark}[The certified margins versus the true margin]
The small margins in Table~\ref{tab:fq1-results} measure the slack of the \emph{relaxations} being certified (the support bound of Lemma~\ref{lem:highbudget} and the dual envelope of Lemma~\ref{lem:dual-splice} are both nearly tight along their splice), not the distance of~\eqref{eq:fiber-inequality} from failure. In the extremal coordinates of Section~\ref{sec:disagreement}, the constant fiber $u\equiv1$ (for which $V=1$ and $\beta=\nu$) \emph{realizes}
\[
        \rho\;=\;\frac{3\nu^2-1}{\nu^2}\;=\;3-\frac{\pi}{2}\;=\;1.42920\ldots,
\]
and numerical scans over the threshold family $(a,\tau)$ found no smaller value, suggesting that $3-\pi/2$ is the true infimum of $\rho$; we neither need nor prove that sharper assertion. The fiber inequality asserts only $\rho\ge1$, so it holds with about $0.43$ of numerical headroom; in particular, the sharper inequality $V\le3\nu\beta-c\beta^2$ appears to hold for every $c<3-\pi/2$, though only $c=1$ is certified and used here.
\end{remark}




% \section{Case study: the lower bound}
% \label{app:ai-case-study}

% The lower bound is the run's main discovery. We reconstruct it here in
% outline, highlighting the three human interventions that shaped it, since
% the weaknesses discussed in Section~\ref{sec:ai-discussion} refer back to
% them; the full logs of the sessions involved will be released with the rest
% of the record.
% % {\color{red}AX: You don't have to refer to to-be-released artifacts here.
% % Tell Fable to write this version as though we're *not* releasing additional artifacts.
% % If and when we release artifacts, we'll strategically insert a few footnotes where needed.
% % }

% % {\color{red}AX: As currently written, I think the current section will be hard to track for anyone *not* intimately involved in the paper.
% % Granted, this is hard because it is about exploring a lot of concepts ...
% % Is it possible to extract a general/high-level for a proof template/sketch/idea so that we can ``set the scene'' + provide context?
% % \\
% % Additionally, I think you could consider adding a brief ``Overview`` paragraph of sorts that someone *not* working on Grothendieck can easily skim and get the big picture. This could be a high-level summarization of the subsequent ``The plateau``, ``First intervention'', etc. paragraphs.
% % }

% \paragraph{The plateau.}
% The run began on the upper bound, searching the limiting-scheme space of our
% preprint for schemes whose correlation function admits a large
% inverse-majorant parameter $\gamma$, since an admissible $\gamma$ gives
% $\KG\le\pi/(2\gamma)$. From the hyperplane value
% $\gamma=\log(1+\sqrt2)\approx0.8814$ it reached $\gamma\approx0.882$, and
% there it stalled: in sessions 12 through 17 it opened six 
% %{\color{red}mechanically distinct escape routes}
% mechanically distinct escape routes, and each failed against the same obstruction,
% namely that cubic coefficient mass cannot be cancelled without also reducing
% the linear coefficient. Each failure was recorded and tagged, and the run's
% response was to begin a seventh variation of the same search.

% \paragraph{First intervention: turn the failures into a theorem.}
% The operators redirected the run in session 18. Instead of attempting another
% escape, it was to synthesize the accumulated failures into a proof that no
% scheme in the class does much better: a ceiling $\gamma\le\Gamma$ valid for
% the full class, with mixtures and arbitrary dimension, converts through the
% optimality theorem of Naor and Regev \cite{naor2014krivine} into the lower
% bound $\KG\ge\pi/(2\Gamma)$. The intervention supplied no new mathematics:
% the problem statement had suggested this dualization from the outset, and
% the run had accumulated exactly the required evidence without making the
% connection. Session 18 identified the Naor--Regev theorem as the correct
% transfer, proved a first ingredient valid in every dimension, and located
% the difficulty precisely: the ceilings it could prove covered too narrow a
% class of schemes.

% \paragraph{Progress in two dimensions.}
% Within days the run had proved a cubic ceiling of strength
% $\Gamma\approx0.8866$ for two-dimensional schemes, with the inequality certified in interval arithmetic, and had sharpened the
% constant numerically to $\Gamma\approx0.8846$. The extension to arbitrary dimension and to mixtures, which the
% duality requires, did not follow: fourteen sessions in the range 32--51
% attacked it, each reducing the gap to a sub-lemma, proving the sub-lemma in
% a restricted setting, and leaving the global assembly open, while the
% restricted results accumulated in memory as apparent progress. Two useful
% facts emerged alongside this loop: the run verified the normalization of the
% Naor--Regev transfer against the original paper, and it computed that
% improving the Davie--Reeds~\cite{Davie1984LowerBoundKG,Reeds1991LowerBoundKG} bound $1.6769566742$ requires a universal ceiling
% only at $\Gamma\le0.93669$, far above the two-dimensional value, so a
% general ceiling could be far from sharp and still give a new lower bound.

% \paragraph{Second intervention: the general bound, through theory.}
% The operators ended this loop with a second redirection, on two grounds:
% refinements of the two-dimensional result were not the object of interest,
% since only a ceiling for the full class dualizes; and the gap was
% conceptual, so further implementation would not close it. The run was to
% spend several sessions on theory alone. Session 55 mapped the dependency
% structure of the preceding weeks and identified the recurring error,
% restricted closures recorded as global progress. Session 56 then produced
% the 
% % {\color{red}decisive (?)} 
% decisive reframe. Every failed transport had been nonlinear in
% quantities that do not average when schemes are mixed; the Hermite
% coefficients $(b_1,b_3)$ of the correlation function, by contrast, are
% linear functionals of the scheme, so a constraint that is affine in
% $(b_1,b_3)$ passes to mixtures and to coefficientwise limits with no further
% argument. Choosing the constraint for transportability, and requiring
% equality at the extremal hyperplane point $(b_1,b_3)=(1,\tfrac16)$, gives
% the one-parameter family of affine constraints
% \[
%         b_3\;\ge\;(1+\lambda)\,b_1-\Bigl(\lambda+\tfrac56\Bigr),
%         \qquad \lambda\ge\tfrac12 ,
% \]
% where $\lambda$ indexes the slope of the line through the hyperplane point.
% Each member forces a barrier $\Gamma_\lambda=(\lambda+\frac56)/(1+\lambda)$
% on the admissible parameter, hence a bound $\KG\ge\pi/(2\Gamma_\lambda)$
% conditional on proving that member, and every $\Gamma_\lambda$ below
% $0.93669$ improves on Davie--Reeds.

% \paragraph{Third intervention: one certified rung before a better one.}
% % \color{red}rung
% The tangent member $\lambda=\tfrac12$, worth $\KG\ge9\pi/16\approx1.767$,
% requires a sharp chaos inequality that remains open, and once the family
% existed the run's inclination was to work toward its strongest provable
% member. The operators set the priority differently: what mattered was to
% establish that the method yields any new lower bound at all, so the run was
% to select a rung whose proof closes, certify it completely, and write it up,
% with improvements inside the family treated as secondary. At $\lambda=1$ the
% proof collapses to elementary structure: session 57 found that the
% decomposition $h=(f+g)/2$, $k=(f-g)/2$ reduces the constraint, fiber by
% one-dimensional fiber, to the ternary inequality~\eqref{eq:fiber-inequality},
% %% TODO: fix cross-reference to the fiber inequality of the lower-bound section
% whose closing case analysis is short, giving $\Gamma_1=\tfrac{11}{12}$ and
% \[
%         \KG\;\ge\;\frac{6\pi}{11}\;\approx\;1.7136 .
% \]
% Sessions 58--64 then subjected the chain to adversarial review, which
% found and repaired the one substantive gap (the passage from finitely many
% schemes to measurable mixtures, closed by a weak-$*$ lemma), a Jensen
% inequality applied in the wrong direction, and a small defect in the
% interval certificate's coverage, after which the run produced the first
% complete write-up, about a day after the reframe. The stronger rungs
% $27\pi/49$ and $51\pi/92$ of Table~\ref{tab:timeline} followed within a week
% by the same method at smaller values of $\lambda$.
